# Supplementary material for: Optimal Representations for Covariate Shift
Source: arXiv:2201.00057 source file (2022-03-14)
Supplement: Supplementary file 1 [file bridge.tex]

\subsection{Bridge setting: understanding what we should do in practice}
\label{main:experiment/bridge}
% Based on the scientific setting, we considered a more practical setting with 
% and motivate the use of CLIP \citep{radford2021learning} models in the following experiments. 
The scientific setup is closer to our theory than what we do in practice in that worst-case predictor was considered and empirical generalization gap was ignored. Here we bridged these gaps with a more practical setup.
In particular, we split the PACS dataset to training and validation splits for each domain and considered the setting: Bob trains the encoder on all-domain training splits with a validation loss selection; Alice trains the SVM predictor (average-case) on the source training split which is selected over the source validation split, and evaluates on the validation splits of other target domains. 
% The ResNet-50 \citep{he2016deep} pretrained on ImageNet \citep{russakovsky2015imagenet} was used as the encoder and the SVM classifier was used as the predictor. 
The target validation accuracy averaged over all (source, target) setups was reported. We will use CAD in following experiments unless otherwise specified (chosen with initial experiments). We repeated the empirical analysis in the scientific setting here and obtained similar results which are included in \cref{appcs:exp_results/bridge}. Here we investigated some remaining empirical questions.

\yrnote{didn't find a good caption for this table..}

\begin{wraptable}{r}{0.45\textwidth}
\vspace{-\baselineskip}
\caption{Comparison on the bridge setting.}
\label{table:bridge_pacs}
\vspace{-\baselineskip}
\begin{center}
\begin{tabular}{l|c}
\toprule
\textbf{Setup} & \textbf{Avg. target acc.}\\
\midrule
CE-Base   &   95.9 $\pm$ 0.5\\ 
CE-CAD     &   96.7 $\pm$ 0.2\\
\midrule
CE-CAD (staggered) & 96.5 $\pm$ 0.0\\
\midrule
SupCon-CAD & 96.7 $\pm$ 0.4 \\
SimCLR-CAD & 61.7 $\pm$ 0.8 \\
\bottomrule
\end{tabular}
\end{center}
\vspace{-2\baselineskip}
\end{wraptable}

\paragraph{Does domain bottleneck improve the average-case DG performance?} 
\yrnote{we might consider removing this}
Though our theory focuses on the worst-case DG, we empirically showed that adding bottlenecks to enforce support match can also improve the average-case DG performance by comparing CE-Base and CE-CAD in \cref{table:bridge_pacs}.

\paragraph{Can we use standard augmentations?}
% Recent SSL models typically adopt standard image augmentations used by SimCLR \citep{chen2020simple}, e.g., cropping and color jittering. 
In \cref{fig:aug}, we point out that standard augmentations are not domain-covering and thus not suitable for SSL with our objectives. We empirically showed this by using augmentations of SimCLR \citep{chen2020simple} with our objectives (SimCLR-CAD).
In \cref{table:bridge_pacs}, we indeed observed that using SimCLR augmentations performed much worse than using desired augmentations (SupCon-CAD). 
% This shows that since SimCLR augmentations are not domain covering, it's harder to enforce support match for the learned representations.
% though SimCLR augmentations are likely to preserve label, they are not domain covering thus more difficult for the learned representations to 

\paragraph{How is end-to-end training compared to staggered training?}
Since getting access to target domain data is not practical in practice, we can utilize SSL models pretrained on a very large support (as we do later). However, typical SSL models are trained without any bottlenecks and we can adopt the staggered training where we freeze the SSL models and train a small network on top with bottlenecks. To get an idea of how it compares to end-to-end training with bottlenecks, we considered a staggered version of CE-CAD in our setup. As shown in \cref{table:bridge_pacs}, it performed similarly to CE-CAD. 
\yrnote{tbh I think this point is not super important, maybe in appcs.. or maybe move to the next section is more natural???}
\yrnote{I didn't rewrite this, tended to move it to appendix, and mentioned it in next section if needed.}
