# Supplementary material for: Optimal Representations for Covariate Shift
Source: arXiv:2201.00057 source file (2022-03-14)
Supplement: Supplementary file 2 [file preliminary_continuous.tex]

\section{Preliminaries}

\subsection{Notation}
\label{appcs:notation}


We assume a background standard probability space that is rich enough to
support all random variables used. We assume that all spaces are standard probability spaces, and, for convenience, the existence of densities. A full list of assumptions is found at \cref{appcs:assumptions}.


\paragraph{General} \tofill{}.
The image of a set $\mathcal{X}$ under a function $f : \inputspace \to \labelspace$ is denoted $\image{f}{B} = \set{f(x) \cond x \in B}$ for $B \subseteq \inputspace$. The pre-image is denoted $\preimage{f}{B} = \set{x \in \inputspace \cond f(x) \in B}$ for $B \subseteq \labelspace$.

\paragraph{Probability} Random variables (r.v.) are denoted by uppercase letters (e.g., $X$), and their sample space and realizations are denoted by the corresponding calligraphic (e.g., $\inputspace$) and lowercase letters (e.g., $x$) respectively. 
The probability distribution of a random variable $X$ is denoted as $\dist{X}$;
the probability density\footnote{In this paper, we refer to the probability density as the probability mass function (pmf) for discrete r.v. or probability density function (pdf) for continuous r.v.} of a random variable $X$ is denoted as $\dens{X}$. The support $\supp{\dist{X}}$ of a distribution is the set of all points $x \in \inputspace$ for which every open neighbourhood $N_x$ of $x$ has positive probability:
\begin{equation}
    \supp{\dist{X}} := \{x \in \inputspace : N_x \ \text{open neighbourhood of} \ x \implies P_X(N_x) > 0 \}
\end{equation}
When it is necessary to be explicit, we will denote `$X$ is distributed as $\dist{X}$' using the notation $X \dsim \dist{X}$ or $X \dsim \dens{X}$.
Expectations are written as: $\E{\dens{X} }{f(X)}$,
independence of two r.v. as $\cdot \indep \cdot$, conditional independence as $\cdot \indep \cdot \cond \cdot$.

For jointly distributed random variables $(X,Y)$ taking value in (t.v.i.) $\inputspace \times \labelspace$, the regular conditional distribution is denoted $\conddist{Y}{X}: \borel{\labelspace} \times \inputspace \to [0, 1]$ and the density is denoted as $\conddens{Y}{X}: \labelspace \times \inputspace \rightarrow [0, \infty)$. Let $\conddist{Y}{x} =  \conddist{Y}{X}( \vardot \cond x)$ be the function of $x$ from $\inputspace$ to the set of all probability distributions on $\labelspace$. Similarly, let $\conddens{Y}{x} = \conddens{Y}{X}( \vardot \cond x)$ be the function of $x$ from $\inputspace$ to the set of all probability densities on $\labelspace$.
% The (regular) conditional density is, 
% \begin{equation}
%     \conddens{Y}{X}(y \cond x)=\conddens{Y}{x}(y)=\frac{\dens{X,Y}(x,y)}{\dens{X}(x)} \for{x \in \supp{\dens{X}}}
% \end{equation}
All random variables are independently distributed, unless an explicit joint distribution or coupling is given.

\subsection{Definitions}
\label{appcs:definitions}

We are interested in prediction problems with domain shift under the covariate shift assumption. There are four random variables: the domain $D$, the input $X$, the label $Y$, and the representation $Z$. They have the following joint distribution:
\begin{equation}
(D, X, Y, Z) \dsim \dens{D} \vardot \conddens{X,Y}{D} \vardot  \conddens{Z}{X}
\end{equation}
where we drop the arguments of the probability densities for clarity. We make a variety of convenience assumptions on these random variables (\cref{asmp:domains}). The key thing to notice here is that $Z$ is conditionally independent of $Y, D$ given $X$. We will be making assumptions on $\dens{D,X,Y}$ that can be thought of as generalized covariate shift assumptions (\cref{asmp:bayes_inv}).

\subsubsection{Risk minimization} 
Our ultimate goal is to predict $Y$ from the representation $Z$ of $X$ in a manner that is robust to changes in the domain. 

We formalize this in the standard way by making predictions  $a \in \actionspace$ in a space of predictions. For example the prediction space may be the set of all possible labels $\actionspace = \labelspace$, in which case we would be predicting deterministic labels. Or we may predict a distribution over labels, in which case the prediction space would be the set of all probability distributions on $\labelspace$, i.e. $\actionspace = \distspace(\labelspace)$.


A \emph{predictor} is a function mapping inputs to predictions or representations to predictions, i.e., $f : \inputspace \to \actionspace$ or $g : \repspace \to \actionspace$. In general, we will use $f$ for predictors from $\inputspace$ and $g$ for predictors from $\repspace$, however, it should also be clear from context. Define the sets of all predictors,
\begin{align}
    \univfamily := \set{f \cond f : \inputspace \to \actionspace}\\
    \univfamilyg := \set{g \cond g : \repspace \to \actionspace}.
\end{align}
For example, $f$ may be a neural network that takes as input a sample $x$ from the encoder and outputs a vector of logits that parameterize a softmax distribution over finitely many labels.

We select predictors according to the \emph{risk} defined via a loss function $\ell : \labelspace \times \actionspace \to \mathbb{R}_{\geq 0} \cup \{\infty\}$:
\begin{align}
  \riskq{Y}{X}{f} \defeq   \E{\dens{X,Y} }{\ell(Y, f(X))}. 
\end{align}
In particular, we are interested in the Bayes (minimum) risk over all predictors:
\begin{equation}
    \label{eq:risk}
    \risk{Y}{X} \defeq \inf_{f \in \univfamily} \riskq{Y}{X}{f},
\end{equation}
We denote the set of all optimal predictors as 
\begin{equation}
\label{eq:optimalpredictors}
\univfamily^* \defeq \set{f \in \univfamily \cond \riskq{Y}{X}{f} = \risk{Y}{X}}
\end{equation}
Similarly, we define the risk $\riskq{Y}{Z}{g}$, the Bayes risk $\risk{Y}{Z}$, and the set of optimal predictors $\univfamilyg^*$ from $Z$. These will all vary as a function of the conditional $\conddist{Y}{Z}$. We assume that together our loss and prediction space always admit optima, and thus $\univfamily^*, \univfamilyg^*$ are always non-empty.


We will be assuming that the risk admits optimal prediction from any representation $Z$ and is uniquely optimized when predicting from $X$ (\cref{asmp:losses}). Thus it makes sense to define the following.

\begin{definition}[The Bayes predictor]
\label{def:bayespredictor}
\emph{The Bayes predictor} $\bayesf : \inputspace \to \actionspace$ is the unique predictor that is optimal for all $x \in \inputspace$:
\begin{equation}
    \bayesf(x) = \arg \min_{a \in \actionspace} \E{\conddens{Y}{x} }{\ell(Y, a)}
\end{equation}
\end{definition}

\begin{definition}[The Bayes image]
\label{def:bayesimage}
The image of all the inputs under the Bayes predictor will be denoted as $\actionspace^* = \image{\bayesf}{\inputspace}$ and called \emph{the Bayes image}.
\end{definition}

% Finally, we may at times be interested in a restricted family of predictors  $\funcfamily \subseteq \univfamily$. In this case, the Bayes (best achievable) risk under the functional family $\funcfamily$ is denoted as
% \begin{equation}
%     \riskQ{Y}{Z} \defeq \inf_{q \in \funcfamily} \riskq{Y}{Z}{q}.
% \end{equation}
% with all the optimal predictors in $\funcfamily$ denoted as $\funcfamily^* \defeq \set{q \in \funcfamily \cond \riskq{Y}{Z}{q} = \riskQ{Y}{Z} }$.


\cmnote{I believe definitions are OK until this point}

\subsubsection{Domain generalization} We are interested in controlling the risk in a domain generalization setting, and so we define \emph{the domain-conditional risk},
\begin{align}
  \domriskq{X}{f}{d} \defeq   \E{\conddist{X,Y}{d} }{\ell(Y, f(X))}.
\end{align}
$\domrisk{X}{d}, \univfamily_d^*$ are defined as \cref{eq:risk,eq:optimalpredictors}, respectively, but with respect to $\operatorname{R}^d_f$. 
Similarly, define the Bayes image for domain $d$ as \begin{equation}
    \actionspace_d^* := \image{\bayesf}{\supp{\conddist{X}{d}}}.
\end{equation}
We also define domain-conditional quantities for prediction from a representation $Z$. The most important term which we will be investigating is an idealization of the domain generalization worst-case risk.

\begin{definition}[IDG Risk]
Given a distribution $\dist{\Dt, \Ds}$ over a target domain $\Dt$ and source domain $\Ds$ t.v.i. the product space $\domspace \times \domspace$, the idealized domain generalization worst-case risk, \textit{IDG risk} for short, is the expected worst-case target risk taken over source minimizers, \ie,
\begin{equation}
 \quad \E{\dist{\Dt, \Ds}}{\sup_{g \in \univfamilyg_{\Ds}^*} \domriskq{Z}{g}{\Dt}}  
\end{equation}
\end{definition}

Note that the IDG risk is well-defined because $\univfamily_{\Ds}^*$ is non-empty as it always contains the Bayes predictor $\dombayesf{\Ds}$ due to \cref{asmp:losses}. The desired optimal representations, are then those that minimize the IDG risk.

\begin{definition}[Optimal representations for idealized domain generalization]
An encoder $\conddist{Z^*}{X}$ is \textit{optimal} for idealized domain generalization if and only if it minimizes the IDG risk, \ie, 
\begin{equation}
 \E{\dist{\Dt, \Ds}}{\sup_{g \in \univfamilyg_{\Ds}^*} \domriskq{Z^*}{g}{\Dt}} =  \inf_{\conddist{Z}{X}} \quad \E{\dist{\Dt, \Ds}}{\sup_{g \in \univfamilyg_{\Ds}^*} \domriskq{Z}{g}{\Dt}}
\end{equation}
\end{definition}

\subsubsection{Augmentations}
\cmnote{I have not read this section, and am skipping it}

\begin{definition}\label{def:augmentation}
Augmentation $A$ \ydnote{write in a way which is understandable what an augmentations is, but for simplicity we will restrict ourselves to augmentations whose codomain is $\supp(p(X))$}
\end{definition}

\begin{definition}
We call $p(\Tilde{Z} | A(X)) \defeq \E{p(\Tilde{X} | X; A)}{p(Z|X=\Tilde{X})}$ the \textit{augmented encoder} resulting from $A$ and  $p(Z|X)$.
\end{definition}

\ydnote{similar tengyu but non weighted }
\begin{definition}
We call the \textit{augmentation graph} the directed graph $\mathcal{G}_A$ whose vertices are $\mathcal{X}$ and $x,x' \in \mathcal{X}$ are connected by an edge $x\to x'$ if and only if one  it is possible to augment from $x$ to $x'$, \ie, $p(x \cond x'; A) > 0$.
\end{definition}


\begin{definition}
We call the \textit{weak connected component in $\mathcal{G}_{A}$} the function $C_A : \mathcal{X} \to 2^{\mathcal{X}}$ that maps $x$ to a set of vertices in $\mathcal{G}_{A}$ that are weakly connected to $x$, \ie, the largest set such that there exists an undirected path from $x$ to any $x' \in C_A(x)$.
Furthermore, we denote as $\mathcal{C}_A \defeq C_A^{\rightarrow}(\mathcal{X})$ the set of all weakly connected components in $\mathcal{G}_{A}$.
\end{definition}

We now have all the tools to define a domain translation.

\begin{definition}
We call an augmentations $A$ a \textit{domain translation} iff:
\begin{itemize}
    \item \textbf{Bayes preserving}:  $f_*(\Tilde{X}) = f_*(X)$ almost surely over $p(\Tilde{X} | X; A)p(X)$.
    \ydnote{need to rephrase}
    \item \textbf{Spans domains}: any weakly connected component of $\mathcal{G}_A$ contains at least one vertex $x$ in each domain. 
    Specifically,  $\forall c \in \mathcal{C}_A$ and $\forall d \in \mathcal{D}$, there exists $x \in \supp{p(X|d)}$ such that $C_A(x) = c$.
\end{itemize}

If the domain span also holds for any strongly connected component of $\mathcal{G}_A$, we call $A$ a strong \textit{domain translation}.
\ydnote{not sure if we'll need strong domain translations}
\end{definition}

% \begin{definition}\label{def:aug_opt}
% We say that an encoder is \textit{optimal for bottleneck self-supervised learning under augmentation $A$} (optimal for $A$-BSSL)
% \ydnote{}

% \end{definition}

\subsection{ Assumptions}
\label{appcs:assumptions}

We make a the following assumptions throughout the paper. \textbf{All these assumptions should hold for practical settings.}

\begin{assumption}[Standard probability spaces]\label{asmp:probabilityspaces}
All spaces $(\domspace, \inputspace, \labelspace, \repspace, \actionspace)$ are standard Borel spaces and that all distributions are complete.This ensures the existence of regular conditional probability distributions. These technical assumptions generally hold for any practical purposes.  Because the distributions of $X, Y, D$ are fixed, we assume for convenience that $\supp{\dist{X}} = \inputspace$, $\supp{\dist{Y}} = \labelspace$, and $\supp{\dist{D}} = \domspace$.
\end{assumption}

\ydnote{We chatted with chris: Let's call that strictly proper instead of meaningful
}
\ydnote{we need to prove that most desired loss satisfy that (at least log loss, MSE, acc)}
\ydnote{Seems that you removed the assumption that I had that $|\mathcal{A}| \geq 2$. I think we need to add it back to avoid trivial strictly proper losses than break all IFF.}
\begin{assumption}[Meaningful and proper losses]\label{asmp:losses}
The prediction space together with our loss are proper and admit unique optimal predictions of $Y$ from $X$. In particular, we assume that
\begin{enumerate}
\item For all $\dist{\Upsilon} \in \distspace(\labelspace)$, there exists $a^* \in \actionspace$ such that
\begin{equation}
    \E{\dist{\Upsilon}}{\ell(\Upsilon, a^*)} \leq \E{\dist{\Upsilon}}{\ell(\Upsilon, a)} \qquad \forall \ a \in \actionspace.
\end{equation}    \item For all $x \in \inputspace$, there exists $a^* \in \actionspace$, such that
\begin{equation}
    \E{\conddist{Y}{x}}{\ell(Y, a^*)} <\E{\conddist{Y}{x}}{\ell(Y, a)} \qquad \forall \ a \neq a^*.
\end{equation}
\end{enumerate}
Note that for log-loss $\ell$ and finite $\labelspace$ these assumptions are satisfied if $\actionspace = \distspace(\labelspace)$ by strict properness \tocite{}. If we consider the 0-1 loss with $\actionspace = \labelspace$ and a finite label space, these assumptions are mostly satisfied, except we assume that $\conddist{Y}{x}$ is not the uniform distribution.
\end{assumption}

%  under the conditional $\conddist{Y}{x}$ for all $x \in \inputspace$ and $d \in \domspace$.
% \yrnote{$\mathcal{P}(\mathcal{Y})$ is not defined now.}
% I.e., for all $a' \in \mathcal{A}$ we have $\E{p(Y)}{\ell (Y, a_*)} \leq \E{p(Y)}{\ell (Y, a')}$ with equality if and only if $a_* = a'$.
% This is the case for any proper scoring rules, \eg, log loss, or typical point-wise loss functions such as mean squared error, mean absolute error,
% 0-1 loss (accuracy), Huber loss.
% \begin{assumption}[Finite risk]\label{asmp:finite_risk}
% We restrict ourselves to tasks $Y$, such that the unconditional risk is finite, \ie, $\inf_{a \in \mathcal{A}} \E{p(Y)}{\ell (Y, a)} < \infty$.
% \end{assumption}

% For MSE that's finite variance , for log loss that's fintie entropy, for accuracy always holds.




% \ydnote{
% define $f_*$ for surely optimal bayes predictor for Z and X.
% }

\begin{assumption}[Properties of the Bayes predictor]\label{asmp:bayes_inv}
The Bayes predictor satisfies the following properties.
\begin{enumerate}
    \item\label{asmp:bayes_inv:measurability} $\bayesf : \inputspace \to \actionspace$ is a measurable function.
    \item\label{asmp:bayes_inv:covshift} For any $f \in \univfamily$, we have $\dist{D}-$a.s.: 
\begin{equation}
    \E{\conddist{X,Y}{d}}{\ell (Y, \bayesf(X))} \leq \E{\conddist{X,Y}{d}}{\ell (Y, f(X))}.
\end{equation}
\end{enumerate}
%\ydnote{Could change to a.s. over $p(D)$ but I don't see the point.}
\cref{asmp:bayes_inv:covshift} is  the core assumption for our theoretical results. For example, in the case of strictly proper scoring rules, covariate shift $\conddens{Y}{X,D} = \conddens{Y}{X}$ guarantees that this holds. For the 0-1 loss, this is guaranteed by invariance of the most likely label which is less stringent than the typical covariate shift assumption.  \tofill{}
\end{assumption}

\begin{assumption}[Constant Bayes image]\label{asmp:image}
The Bayes image is invariant across domains: \begin{equation}
    \actionspace_d^* \distaseq{\dist{D}} \actionspace^*.
\end{equation}
For the case of accuracy, this simply means that the label set for all domains is the same, while for log-loss this means that the set of possible conditional distributions is the same across domains.
\end{assumption}
\ydnote{Should be 
$supp(f_\# (X|d) ) = f_\# supp( (X|d) ) = supp(f_\# (X) ) = f_\# supp( (X) )$. 
We actually only need $supp(f_\# (X|d) )  = supp(f_\# (X) ) $ but making the 4 equalities just ensure that no annoying measure zero thing ever arises.
}

\begin{assumption}[Embedding the predictions]
\label{asmp:embedding}
There exists an embedding $\phi : \actionspace^* \to \repspace$ such that
\begin{enumerate}
    \item $\phi$ is measurable and one-to-one.
    \item \label{item:openembedding} The support of the pushforward measures $\pushforward{(\phi \circ \bayesf)}{\dist{X}}$ and $\pushforward{(\phi \circ \bayesf)}{\conddist{X}{d}}$ are the images of the supports:
    \begin{equation}
        \begin{aligned}
            \supp{\pushforward{(\phi \circ \bayesf)}{\dist{X}}} &= \image{(\phi \circ \bayesf)}{\supp{\dist{X}}}\\
            \supp{\pushforward{(\phi \circ \bayesf)}{\conddist{X}{d}}} &\distaseq{\dist{D}} \image{(\phi \circ \bayesf)}{\supp{\conddist{X}{d}}}
        \end{aligned}
    \end{equation}
    \ydnote{trivial once we change constant bayes image assumption to $supp(f_\# (X|d) )  = supp(f_\# (X) ) $}
\end{enumerate}
% For example, if $\inputspace$ is a discrete set with the discrete topology, then \cref{item:continuousembedding} is automatically satisfied. If $\inputspace = \mathbb{R}^n$ with the usual topology, then \cref{item:continuousembedding} requires that the composition $\phi \circ \bayesf$ is continuous in the usual sense.
\end{assumption}

% \begin{assumption}[Cardinality of $|\mathcal{Z}| \geq |\mathcal{A}_*|$]\label{asmp:cardinality}
% We assume that the cardinality of the considered sample space $\mathcal{Z}$ is larger than the Bayes image. 
% This ensures that the optimal representation always exists.
% \tofill{}
% \end{assumption}



\begin{assumption}[Domain marginal ]\label{asmp:domains}
$\dist{\Dt, \Ds}$ is any distribution such that 
$\dist{\Dt} = \dist{\Ds} = \dist{D}$.
\end{assumption}



\begin{assumption}[Convenience assumption: Existence of densities]
\label{asmp:density_exist}
Throughout the paper we assume the existence of (conditional) probability mass/density function with respect to some underlying measure.
This assumption is not necessarily needed everywhere, but it simplifies the notation and discussion. 
\end{assumption}









% \subsection{Overview}
% \ydimp{Most of that will be repeated in the main paper so we should jsut cut short and have the notation defined in previous section.}
% \ydimp{Didn not modify that}



% We are interested in prediction problems with domain shift under the covariate shift assumption. In this subsection we give an overview of the problem and our main result in somewhat informal terms. In the next section, we give formal statements of our assumptions, our main theorems, and our proofs.


% \paragraph{The random variables of interest.} 
% % \yrnote{probably put in main body}
% We are interested in predicting a random variable $Y$ (the label) from a random variable $X$ (the input). We also assume that there is a domain random variable $D$, which describes the distribution shift in the prediction problem. Finally, our goal in this paper is to optimize over the possible representations of $X$. So, we introduce a representation random variable $Z$, which is induced by a (stochastic) encoder $\conddist{Z}{X}$. We make the following factorization assumption on their joint distribution:
% \begin{equation}
% (D, X, Y, Z) \dsim \dens{D} \vardot \conddens{X,Y}{D} \vardot  \conddens{Z}{X}
% \end{equation}
% where we drop the arguments of the probability densities for clarity. To unpack this more explicitly:
% \begin{enumerate}
%     \item $Z$ is conditionally independent of $(Y, D)$ knowing $X$.
% \end{enumerate}




% \paragraph{Risk minimization}
% Our goal is characterize the optimal representations for domain generalization, so we are interested in minimizing the risk of predicting the label $Y$ from the representation $Z$ of $X$. More precisely, a predictor $q: \repspace \to \mathcal{A}$ is a mapping from $\repspace$ into the set $\distspace(\labelspace)$ of densities over $\labelspace$ that we use to predict the labels. For discrete label $Y$, the log loss (for classification) is used for specifying the risk: 
% \begin{align}
%   \riskq{Y}{Z}{q} \defeq   \E{\dens{Z,Y} }{- \log  q(Y \cond Z)}. 
% \end{align}
% We denote the predictor functional family as $\funcfamily \subseteq \univfamily = \set{q \cond q : \repspace \to \distspace(\labelspace) }$, where $\univfamily$ denotes the largest (or \emph{universal}) functional family. The Bayes (best achievable) risk under the functional family $\funcfamily$ is denoted as
% \begin{equation}
%     \riskQ{Y}{Z} \defeq \inf_{q \in \funcfamily} \riskq{Y}{Z}{q}.
% \end{equation}
% with all the optimal predictors in $\funcfamily$ denoted as $\funcfamily^* \defeq \set{q \in \funcfamily \cond \riskq{Y}{X}{q} = \riskQ{Y}{X} }$. Similarly, given $D=d$, we can define the domain-conditional risk,
% \begin{align}
%   \domriskq{Z}{q}{d} \defeq   \E{\conddist{Z,Y}{d} }{- \log  q(Y \cond Z)};
% \end{align}
% the domain-conditional Bayes risk, $\domriskQ{Y}{Z}{d} \defeq \inf_{q \in \funcfamily} \domriskq{Z}{q}{d}$; and the domain-conditional optimal predictors, $\funcfamily_d^* \defeq \set{q \in \funcfamily \cond \domriskq{Z}{q}{d} = \domriskQ{Y}{Z}{d}}$.

% \paragraph{Problem statement}
% Consider a distribution $\dist{\Ds, \Dt}$ over two domain random variables, the source $\Ds$ and the target $\Dt$. Our goal is to character the set of encoders $\conddist{Z}{X}$ that minimize the worst case risk on the target domain when selecting predictors from the set of optimal source predictors:
% \begin{align} \label{eq:full_gen_risk_obj}
%     \inf_{\conddist{Z}{X}} \quad 
%     & \E{\dist{\Ds, \Dt}}{  \sup_{q \in \funcfamily_{\Ds}^* }  \domriskq{Z}{q}{\Dt}}.
% \end{align}
% \cmnote{I realized that there is a potential crucial mistake in our reasoning. Basically $\funcfamily_{\Ds}^* $ may be an empty set. So we can either patch this up with more assumptions, or move to universal family.}
% We call such encoders, the optimal encoders for idealized domain generalization. Our main result is a characterization of the optimal encoders for idealized domain generalization.


% \begin{theorem*}[Full Theorem, Informal]
% Under a suitable set of assumptions, there exists an optimal encoder for idealized domain generalization, \cref{eq:full_gen_risk_obj}. Moreoever, an encoder $\conddist{Z}{X}$ achieves the minimum of
% \begin{align}
%     \min_{\conddist{Z}{X}} \quad  \E{\dens{\Ds, \Dt}}{  \sup_{q \in \funcfamily_{\Ds}^* }  \domriskq{Z}{q}{\Dt}}.
% \end{align}
% if and only if it achieves the minimum of
% \begin{align}
% \min_{\conddist{Z}{X}} \quad& \riskQ{Y}{Z} \label{eq:full_iff_min_risk}   \\
% &\subject \quad \supp{\conddist{Z}{d}} \distaseq{\dist{D}} \supp{\dist{Z}}.  \label{eq:full_iff_support_match}  
% \end{align}
% \end{theorem*}

% \begin{remark}
% In fact, we will show that the minimum of \cref{eq:full_iff_min_risk} under the constraint \cref{eq:full_iff_support_match} can still achieve the (unconstrained) best possible risk, i.e., $\inf_{\conddist{Z'}{X}} \riskQ{Y}{Z'}$. Thus the optimality condition can also be rewritten as two constraints: 
% \begin{gather}
%     \riskQ{Y}{Z} = \inf_{\conddist{Z'}{X}} \riskQ{Y}{Z'} \\
%     \supp{\conddist{Z}{d}} \distaseq{\dist{D}} \supp{\dist{Z}}. 
% \end{gather}
% which forms the starting point our proof strategy. But we still keep the optimization form as in \cref{eq:full_iff_min_risk} because it leads to the practical optimization for achieving the optimal representations.
% \end{remark}
