# Supplementary material for: Optimal Representations for Covariate Shift
Source: arXiv:2201.00057 source file (2022-03-14)
Supplement: Supplementary file 3 [file preliminary_old.tex]

\section{Preliminaries}

\subsection{Notation}

Random variables (r.v.) are denoted by uppercase letters (e.g., $X$), and their sample space and realizations are denoted by the corresponding calligraphic (e.g., $\inputspace$) and lowercase letters (e.g., $x$) respectively. We assume that all spaces are standard probability spaces throughout.

The probability distribution of a random variable $X$ is denoted as $\dist{X}$;
The probability density\footnote{In this paper, we refer to the probability density as the probability mass function (pmf) for discrete r.v. or probability density function (pdf) for continuous r.v.} of a random variable $X$ is denoted as $\dens{X}$. The support $\supp{\dens{X}}$ of $X$ is smallest closed set $B$ in the Borel $\sigma$-algebra such that $P_X(B) = 1$.
When it is necessary to be explicit, we will denote `$X$ is distributed as $\dens{X}$' using the notation $X \dsim \dens{X}$. 

For jointly distributed random variables $(X,Y)$ taking value in (t.v.i.) $\inputspace \times \labelspace$, the conditional density is denoted as $\conddens{Y}{X}:\supp{\dens{X}} \rightarrow \distspace(\labelspace)$, where $\distspace(\labelspace)$ denotes all probability densities on $\labelspace$, and its image of $x$ is denoted as $\conddens{Y}{x}=\conddens{Y}{X}( \vardot \cond x)\in\distspace(\labelspace)$. The (regular) conditional density is, 
\begin{equation}
    \conddens{Y}{X}(y \cond x)=\conddens{Y}{x}(y)=\frac{\dens{X,Y}(x,y)}{\dens{X}(x)} \for{x \in \supp{\dens{X}}}
\end{equation}
All random variables are independently distributed, unless an explicit joint distribution or coupling is given.

\subsection{Definitions}
\begin{definition}[Alignment of conditionals]\label{def:cond_align}
% \ydnote{changed slightly: as a matter of style I like when it's written both in english and in math (and then with the math you can be more formal).}
We say that two conditional distributions \emph{align}  $\conddens{Y}{X}\condalign\conddens{Y'}{X'}$ if they are equal on the intersection of their support, \ie, 
% \ydnote{I'd be tempted to put only the prime on X, i.e., $\conddens{Y}{X'}$ but don't feel strongly}
\begin{equation}
   \forall x \in \supp{\dens{X}}\bigcap\supp{\dens{X'}}, \  
   \conddens{Y}{X}(\vardot \cond x)=\conddens{Y'}{X'} (\vardot \cond x)
\end{equation}
The properties of the align relation include:
\begin{itemize}
    \item \textbf{reflexivity}: $\conddens{Y}{X} \condalign \conddens{Y}{X}$
    \item \textbf{symmetry}: $\conddens{Y}{X}\condalign\conddens{Y'}{X'} \iff \conddens{Y'}{X'}\condalign\conddens{Y}{X}$
    \item \textbf{partial transitivity}: if $\conddens{Y}{X}\condalign\conddens{Y'}{X'}$ and $\conddens{Y}{X}\condalign\conddens{Y''}{X''}$, then  $\conddens{Y'}{X'}\condalign\conddens{Y''}{X''}$ \emph{if} $\supp{\dens{X''}} \subseteq \supp{\dens{X}}$ or $\supp{\dens{X'}} \subseteq \supp{\dens{X}}$.
    % \ydnote{haven't seen any use of these properties that are useful in the proofs.
    % Also I would call it ``partial transifitivity'' or ``subset transitivity''.
    % Transitivity is something well defined, and because of that it makes it seem that ``align'' is an equivalence relation which is not true.
    % }
\end{itemize}
\end{definition}


\paragraph{Domain shift} 
% \yrnote{probably put in main body}
In this paper, we are interested in prediction in the the domain shift setting under the covariate shift assumption. 

In particular, we are interested in a collection of prediction problems $(X_d, Y_d)$ indexed by a domain index $d \in \domspace$ where $\domspace$ is the domain space (a discrete set in our setting). $X_d$ is the input for domain $d$ and our goal is to predict its label $Y_d$. We will make use of a representation $Z_d$, which is induced by a (stochastic) encoder $\conddens{Z_d}{X_d}$. 
For all $d \in \domspace$, the triple $(X_d, Y_d, Z_d)$ is distributed as
% \ydnote{huh ?? this reads like $X_d$ mutually independent of $ Z_d$.
% I suppose you mean independence between the triplets from different domains, but that's not true right ? if you have highly correlated domains then they are not independent right ?
% }
\begin{align}
(X_d, Y_d, Z_d) &\dsim \dens{X_d} \vardot  \conddens{Y_d}{X_d} \vardot  \conddens{Z_d}{X_d}
\end{align}
where we drop the arguments of the probability densities for clarity.
% \ydnote{In the appendices I would really like to separate notation from our setting (in the paper it's better not to: much easier to read).
% Btw when ``dropping arguments'' usually statisticians use a different multiplication $P_X \bigotimes P_{Y|X} $ as in \url{https://arxiv.org/pdf/2012.14868.pdf}. Not sayign we have to, but just saying.
% }

We will also make use of domain-marginalized random variables $(X, Y, Z)$, whose joint density is:
\begin{align}
    \dens{X, Y, Z}(x, y, z) = \sum_{d \in \domspace} \dens{D}(d) \dens{X_d}(x)\conddens{Y_d}{X_d}(y | x) \conddens{Z_d}{X_d}(z | x).
\end{align}
\ydnote{
I would change the notation everywhere by using conditionals instead of subscripts for the densities, e.g., $p_{X_d} = p_{X|d}$. So that would become: $\dens{X, Y, Z}(x, y, z) = \sum_{d \in \domspace} p_D(d) p_{X|D}(x|d) p_{Y|X,D}(y|x,d) p_{Y|X,D}(y|x,d)$.
2 reasons:
1/ at some point we might want to drop the subscripts on $p$ to avoid cluttering, current notation doesn't allow that.
2/ it's more standard.
3/ it makes it more obvious that you can use standard rules of probability: $p_(D)(d) p_{X|D}(x|d) = p_{X,D}(x,d)$ is obvious to anyone without needed context. $p_{D}(d) p_{X_d}(x) = p_{X,D}(x,d)$ not obvious at all without more context (people do pattern matching: you multiply by what you condition means that you get a joint).
Then we just say ``for notational convenience we use $X_d \dsim p(X|d)$''.  
}
where $\dens{D}$ is a distribution over domains. 
\ydnote{Let's not use prior to really mean distribution. Trust me that would annoy hard core Bayesian ML people (eg Cambridge students). Prior implies there's a posterior over domains.
}

\begin{definition}(Alignment across domains)\label{def:cond_domain_align}
Given a set of random variables $\{(U_d, V_d)\}_{d \in \domspace}$, we say that the domain conditionals $\conddens{U_d}{V_d}$ `align across domains', if they all align with the domain-marginalize conditional,
\begin{equation}
    \conddens{U_d}{V_d} \condalign \conddens{U}{V}, \, \forall{d \in \domspace}
\end{equation}
where $\dens{U, V}(u, v) = \sum_{d \in \domspace} \dens{D}(d) \dens{U_d, V_d}(u, v)$. Note that then they align with each other by transitivity.
\end{definition}
% \ydnote{If we only use $U=Y$ then use $Y$ instead of $Y$. 
% }
% \ydnote{Also I would be tempted to keep ``covariate shift'' as we did until now: the more you use previous terms in the literature the higher the chance for skimmers to understand your results.}

% The key technical assumptions the we make on these random variables is that the conditionals $\conddens{Y_d}{X_d}$ and $\conddens{Z_d}{X_d}$ align across domains. We will also show that for optimal representations, the conditionals $\conddens{Y_d}{Z_d}$ also align across domains.

 We make two key assumptions to the data generating process:
\begin{enumerate}
    \item  We assume \textbf{covariate shift} (\cref{asmp:covariate_shift}), which means that $\conddens{Y_d}{X_d}$ align across domains.
    \item We assume the same (stochastic) encoder used for all domains, which means that $\conddens{Z_d}{X_d}$ align across domains.
\end{enumerate}

% Based on these two assumptions, the joint distribution of $(X_d, Y_d, Z_d)$ can also be rewritten as:
% \begin{align}
% (X_d, Y_d, Z_d) &\dsim \dens{X_d} \vardot  \conddens{Y}{X} \vardot  \conddens{Z}{X}
% \end{align}

% $Y$ is a label drawn from a conditional $\conddens{Y}{X}$. $Z$ is the representation drawn from a conditional $\conddens{Z}{X}$. They are jointly distributed as,
% \begin{align}
% (X, Y, Z) &\dsim \dens{X} \vardot  \conddens{Y}{X} \vardot  \conddens{Z}{X}
% \end{align}

%  In particular,
% \begin{enumerate}
%     \item  We assume \textbf{covariate shift} (\cref{asmp:covariate_shift}), which is the assumption that $\conddens{Y}{X} \condalign \conddens{Y_d}{X_d}$ for all $d \in \domspace$.
%     \item We assume the same (stochastic) encoder for all domains, which is the assumption that $\conddens{Z}{X} \condalign \conddens{Z_d}{X_d}$ for all $d \in \domspace$.
% \end{enumerate}
% Based on these two assumptions, the joint distribution of $(X_d, Y_d, Z_d)$ can also be rewritten as:
% \begin{align}
% (X_d, Y_d, Z_d) &\dsim \dens{X_d} \vardot  \conddens{Y}{X} \vardot  \conddens{Z}{X}
% \end{align}


% \begin{align}
% D, X, Y, Z &\dsim \dens{D} \vardot \conddens{X}{D} \vardot \conddens{Y}{X} \vardot  \conddens{Z}{X}
% \end{align}





% In particular, denote $X, Y$ as the input and label which t.v.i. $\inputspace, \labelspace$, respectively., and it t.v.i. $\repspace$. $D$ is the domain and its space $\domspace$ is typically a set of integer-valued indices. 
% The joint distribution is
% \begin{align}
% D, X, Y, Z &\dsim \dens{D} \vardot \conddens{X}{D} \vardot \conddens{Y}{X} \vardot  \conddens{Z}{X}
% \end{align}
% For convenience, we also define random variables $X_d, Y_d, Z_d$, which are the random variables $X, Y, Z$ conditioned on being in a specific domain $d$, i.e.,  
% \begin{align}
% X_d, Y_d, Z_d &\dsim \dens{X_d} \vardot  \conddens{Y}{X} \vardot  \conddens{Z}{X}
% \end{align}
% where $\dens{X_d}\defeq\conddens{X}{D}(\vardot \cond d)$. Note that the covariate shift assumption can be rewritten as $\conddens{Y}{X} \condalign \conddens{Y_d}{X_d}$. 

\paragraph{Risk minimization}
Given the representation $Z$, a predictor $q: \repspace \to \distspace(\labelspace)$ is used to predict the distribution over the labels. For discrete label $Y$, the log loss (for classification) is used for specifying the risk: 
\begin{align}
   \riskq{Y}{Z}{q} \defeq  \E{\dens{X,Y} \vardot \conddens{Z}{X}}{- \log  q(Y \cond Z)} =  \E{\dens{Z,Y} }{- \log  q(Y \cond Z)}. 
\end{align}
Denote the predictor functional family we can use as $\funcfamily \subseteq \univfamily = \set{q \cond q : \repspace \to \distspace(\labelspace) }$, where $\univfamily$ denotes the largest (or \emph{universal}) functional family. The Bayes (best achievable) risk under the functional family $\funcfamily$ is denoted as
\begin{equation}
    \riskQ{Y}{Z} \defeq \inf_{q \in \funcfamily} \riskq{Y}{Z}{q}.
\end{equation}
with all the optimal predictors in $\funcfamily$ denoted as $\funcfamily^* \defeq \set{q \in \funcfamily \cond \riskq{Y}{X}{q} = \riskQ{Y}{X} }$. Similarly we can define the Bayes risk of a specific domain $d$ as $\riskQ{Y_d}{Z_d} \defeq \inf_{q \in \funcfamily} \riskq{Y_d}{Z_d}{q}$ with optimal predictors $\funcfamily_d^* \defeq \set{q \in \funcfamily \cond \riskq{Y_d}{X_d}{q} = \riskQ{Y_d}{X_d} }$.

\paragraph{Problem statement}
\yrnote{will move to main body}
We consider the problem of learning optimal representations for domain shift without knowing the source and target domains ahead of time. In particular, we assume the (labeled) `source' domain $\Ds$ and the (unlabeled) `target' domain $\Dt$ are randomly selected from $\dens{D}$ i.i.d., and we want to find an encoder $\conddens{Z}{X}$ to minimize the expected generalization risk from $\Ds$ to $\Dt$. To provide guarantees of any predictor selected on $\Ds$, we consider the \emph{worst-case} performance of source predictors on target, i.e., $\sup_{q \in \funcfamily_{\Ds}^* } \riskq{Y_{\Dt}}{Z_{\Dt}}{q}$, compared to the best possible target risk, i.e.,
$\inf_{\conddens{Z'}{X}}\riskQ{Y_{\Dt}}{Z'_{\Dt}}$. Our goal is to obtain the encoder $\conddens{Z}{X}$ to minimize the following objective:
\begin{align} \label{eq:full_gen_risk_obj}
    \inf_{\conddens{Z}{X}} \quad 
    & \E{\dens{\Ds, \Dt}}{  \sup_{q \in \funcfamily_{\Ds}^* } \riskq{Y_{\Dt}}{Z_{\Dt}}{q}-  \inf_{\conddens{Z'}{X}}\riskQ{Y_{\Dt}}{Z'_{\Dt}} }
\end{align}
% \ydnote{Changed the first to inf: getting the min is a result not problem statement.}
which we call the `omnidirectional generalization risk' which takes expectation over all possible pairs of source and target domains. Note that $\dens{\Ds, \Dt}(\ds, \dt)=\dens{D}(\ds)\dens{D}(\dt), \forall{\ds, \dt \in \domspace}$.
\ydnote{Why omnidirectlyional generalization risk ?
Deos that term include $inf_{p_{Z|X}}$ (as currently implied)? if so I think it doesn't make sense. If you mean inside the inf, then I would just call it ``excess domain generalization risk'' or something that includes domain.
}
\yrnote{will need to change this name}


\subsection{General Assumptions}
In this subsection, we describe the general assumptions that we make throughout the paper for our theoretical results with brief explanations about why we make these assumptions and why these assumptions can hold in practice. 

\begin{assumption}[Discrete and finite labels]\label{asmp:discrete_label}
We consider classification tasks where the label $Y$ is discrete and its space $\labelspace$ is finite. For $X$, $Z$, we do not restrict them to discrete or continuous.
\yrnote{be more careful about this}
\end{assumption}
% \ydnote{double check that we don’t need “finite” labels (can we deal with countable as assumption suggests). I'd be fine saying finite $\mathcal{Y}$ which is natural for classification. }
\ydnote{$X$, $Z$ should not be in that assumption}

\begin{assumption}[Discrete and finite domains]\label{asmp:finite_domain}
\yrnote{probably remove this}
\ydnote{now that we want to deal with domain generalization rather than domain adaptation this is slightly strange, because really what we want to say is provide guarantees to any domains whose support is a subset of the joint support + covariate shift.

I think infinite $\mathcal{D}$ might be a mess though, so I would probably do finite + add an additional proposition or note ``btw our optimal representation provides guarantees for any domains that ...''.
}
We assume that $D$ is discrete and its sample space $\domspace$ is finite. This assumption is made to avoid the need to consider countably infinite domains in the proofs. Although it may not always be true, e.g., one can define countably infinite domains by introducing any possible distribution over $\inputspace$, 
\ydnote{actually that would give uncountably many domains not countable}
it should generally hold in practice since we typically only get access to a finite set of domains. 
\end{assumption}


\begin{assumption}[Full coverage of domains]\label{asmp:cover_domains}
We assume that every domain is sampled with a non-zero probability. Formally, $\forall d \in \domspace, \dens{D}(d) > 0$. This ensures that no domain is never sampled such that we can never put theoretical guarantee on it. Note that this assumption is trivial in practice, e.g., a common choice is to set $\dens{D}$ as a uniform distribution  over $\domspace$.

\end{assumption}

\begin{assumption}[Existence of regular conditional probabilities] 
We restrict ourselves to standard
Borel measurable spaces, so that the existence of regular conditional probability distributions is
ensured. This technical assumption generally holds for any practical purposes. 
\end{assumption}

\begin{assumption}[Convenience assumption: Existence of densities] Throughout the paper
we assume the existence of (conditional) probability mass/density function, \ie, to probability distributions that are absolutely continuous with respect to the underlying measure.
This assumption is not needed but simplifies the notation and ensures that we can work with the support of the densities instead of using ``almost sure'' statements. 
\end{assumption}
% \ydnote{I splitted assumptions}

\begin{assumption}[Covariate shift]\label{asmp:covariate_shift}
This is the core assumption for our theoretical results. We assume that the conditional $\conddens{Y_d}{X_d}$ align across domains (\cref{def:cond_domain_align}) and only the marginal $\dens{X_d}$ change across domains. This assumption ensures the existence of optimal representations for domain shift and is commonly made in a bunch of domain generalization/adaptation literature \tocite{}.
\end{assumption}
