# Supplementary material for: Optimal Representations for Covariate Shift
Source: arXiv:2201.00057 source file (2022-03-14)
Supplement: Supplementary file 4 [file theory_continuous.tex]

\section{Proofs}

\subsection{Proof of \Cref{thm:main}}

\ydnote{We will now deal only with finite in main paper, and have a section in appcs that state the theorems and show how to extend the proofs (and which assumptions) for continuous. 
The proofs will then not be very detailed.
The goal of this section is:
(1) to show that the results are not an artefact from working in finite spaces;
(2) provide the full statement of the theorem;
(3) give an intuition as to how to prove it.
We should look at tengyu's paper on augmentations / SSL to get an idea as to how theoreticians would write such a section.
}

An important result that we will be using is the generalized data processing inequality of Bayes risk \cite{xu_minimum_2020,dubois2021lossy}.
We include it here for
completeness.

\begin{lemma}[Generalized DPI \cite{xu_minimum_2020,dubois2021lossy}]\label{lem:DPI}
Let $Z-X-Y$ be a Markov chain of random variables. For any loss function $\ell$,
\begin{equation}
\risk{Y}{X} \leq \risk{Y}{Z}.
\end{equation}
\end{lemma}

For the case of meaningful losses we can go one step further and prove a generalized conditional mutual information identity. Note that we prove the lemma without using any finiteness assumption, as this could be useful for future work.

\begin{lemma}[Generalized CMI]\label{lem:CMI}
 \ydnote{Maybe instead of introducing a new letter for all bayes predictor, we should do like in lossyless: $\psi_{Z}$ is Bayes for Z, while $\psi_{X}$ is Bayes for X}
 Let $\psi_{X,Z}$ denote the Bayes predictor from $(X,Z)$ to $Y$, $\psi_{X}$ is defined similarly from $X$. 
 Assume that the Bayes predictors are measurable.
 For any meaningful loss $\ell$, the \textit{generalized conditional mutual information} is zero if and only if the Bayes prediction are independent of the inputs conditioned on $Z$. Specifically,
\begin{equation}\label{eq:CMI_ZX}
\MIL{Y}{X|Z} \defeq \risk{Y}{Z} - \risk{Y}{X,Z} = 0 \quad \iff \quad 
\psi_{X,Z}(X,Z) \indep X \cond Z
\end{equation}
In particular, if $Y \indep Z \cond X$ then 
\begin{equation}\label{eq:CMI_X}
 \risk{Y}{Z} = \risk{Y}{X}  \quad \iff \quad 
\psi_{X}(X) \distaseq{p(Z,X)} \psi_{Z}(Z)
\end{equation}
\ydnote{Writing the full lemma even though we only use part of it, because we introduce meaningful losses and thus will be useful for future work to have the properties also.}
\end{lemma}
\begin{proof}
Note that we have:
\begin{align}
\risk{Y}{X,Z} &\defeq
\E{p(Y,X,Z)}{\ell(Y,\psi_{X,Z}(X,Z))} \\
&\leq \E{p(Y,Z)}{\ell(Y,\psi_{Z}(Z))} & \text{\cref{lem:DPI}} 
\end{align}
The last equation uses the fact that the predictor $\psi_{X,Z}(X,Z)$ can disregard $X$ and thus always achieve the same risk as $\psi_{Z}(Z)$ (also seen using \cref{lem:DPI} with Markov Chain $Z - (Z,X)- Y$).

As $\ell$ is a strictly proper loss we have equality if and only if  $\psi_{X,Z}(X,Z) \aseq \psi_{Z}(Z)$.
The latter is equivalent to $\psi_{X,Z}(X,Z) \indep X \cond Z$ due to the characterization of conditional independence ( Prop. 5.13 in \citet{kallenberg_foundations_2002}).
Indeed, as a reminder $\psi_{X,Z}(X,Z) \indep X \cond Z$ is equivalent to saying that there exists a measurable function $h$ s.t. $\psi_{X,Z}(X,Z) \aseq h(Z,U)$ with $U \dsim \text{Unif}([0,1])$ and $U \indep (X,Z)$.
The independence of $U$ means that $\psi_{X,Z}(X,Z) \aseq h(Z,u)$ for any $u \in [0,1]$, so setting $\phi_Z(\argdot) = h(\argdot,u)$ concludes the proof of \cref{eq:CMI_ZX}.


Finally, if $Y \indep Z \cond X$ we have $\risk{Y}{X} = \risk{Y}{Z,X}$ by using \cref{lem:DPI} with both Markov Chains $Y - (Z,X) -  X$ and $Y - X - (Z,X)$.
We can thus replace $\risk{Y}{Z,X}$ by $ \risk{Y}{X}$ and $\psi_{X,Z}(X,Z)$ by $\psi_X(X)$ to get $\psi_{X}(X) \aseq \psi_{Z}(Z)$ as desired in \cref{eq:CMI_X}. 
\end{proof}

First we will show that the desired representation exists by taking all example for which the Bayes predictor predicts similarly and ``bucketing'' them to the same representation.
This is a direct extension of the example from \citepos{dubois2020dib} Proposition 6, to the case of meaningful losses.


\begin{lemma}[Existence]\label{lem:exists}
Under our assumptions, there exists an encoder $\conddist{Z^*}{X}$ that such that
\begin{align}\label{eq:lem_min_risk}
\risk{Y}{X} = \risk{Y}{Z^*} \quad \subject \quad \supp{\conddist{Z^*}{d}} \distaseq{\dist{D}} \supp{\dist{Z^*}}.
\end{align}
Because $\risk{Y}{X}$ is the minimum achievable risk by any encoder, $\conddist{Z^*}{X}$ is optimal for the problem in \cref{eq:min_risk,eq:support_match}. This means that all optimal encoders must achieve the Bayes risk $\risk{Y}{X}$.
\end{lemma}

\begin{proof}
Because we assume arbitrary encoders $\conddist{Z}{X}$, the essence of this construction is simple: we embed the prediction space into $\repspace$. Indeed, let $\phi : \actionspace^* \to \repspace$ be any one-to-one measurable function that satisfies \cref{asmp:embedding}. 
Then let $Z^* = \phi(\bayesf(X))$. Note that marginal distribution $\dist{Z^*}$ is a complete measure on a standard Borel space\cmnote{double check this}, and so it satisfies \cref{asmp:domains}. We now verify the properties of $Z^*$.

% \yrnote{I guess a definition/remark between Bayes risk and Bayes predictor is missing, which makes it a bit hard to follow.}
\begin{enumerate}
    \item $Z^*$ satisfies $\risk{Y}{X} = \risk{Y}{Z^*}$. Indeed, 
    \begin{align}
        \risk{Y}{X} &= \E{\dist{X,Y}}{\ell(Y, \bayesf(X))}\\
        &= \E{\dist{X,Y}\conddist{Z^*}{X}}{\ell(Y, f^*(X))} \\
        &\label{eq:bydefzstar} = \E{\dist{Z^*,Y}}{\ell(Y, \phi^{-1}(Z^*))} \\
        &\label{eq:bybayesrisk}\geq \risk{Y}{Z^*}.
    \end{align}
     \cref{eq:bydefzstar} is by our construction of $Z^*$ and \cref{eq:bybayesrisk} is by the definition of the Bayes risk. Due to the data processing inequality of Bayes risk (\cref{lem:DPI}) we also have $\risk{Y}{X} \leq \risk{Y}{Z^*}$, from which we conclude that $\risk{Y}{X} = \risk{Y}{Z^*}$ and that \cref{eq:min_risk} holds regardless of the constraint.
     \item Now let us compute the desired support. By \cref{asmp:image} have that:
     \begin{equation}
     \image{\bayesf}{\supp{\conddist{X}{d}}} = \actionspace^*_d \distaseq{\dist{D}} \actionspace^* = \image{\bayesf}{\inputspace}.    
     \end{equation}
     This, together with \cref{asmp:embedding} means that we have: 
     \begin{align}
         \supp{\conddist{Z^*}{d}} &\distaseq{\dist{D}} \image{(\phi \circ \bayesf)}{\supp{\conddist{X}{d}}}\\
         &\distaseq{\dist{D}} \label{eq:byinvarimage} \image{(\phi \circ \bayesf)}{\inputspace}\\
         &= \supp{\dist{Z^*}}.
     \end{align}
     \cmnote{This argument is ugly AF, because it is purely by assumption. We need to give examples where this is satisfied.}
     \ydnote{trivial once we assume $supp(f_\# (X|d) )  = supp(f_\# (X) ) $}
\end{enumerate}
\end{proof}

% As a direct corollary of the proof we have that $\min \risk{Y}{Z} = \risk{Y}{X}$ under the support constraint
% \ydnote{simple but use multiple times}
% \begin{lemma}[Min risk]\label{lem:min_risk}
% Minimizing \cref{eq:min_risk} under \cref{eq:support_match} gives $\risk{Y}{X}$, \ie,
% \begin{align}\label{eq:lem_min_risk}
% \risk{Y}{X} = &\min_{p(Z \cond X)} \quad \risk{Y}{Z}   \\
% & \subject \quad \supp{p(Z \cond \Ds)} \aseq \supp{p(Z \cond \Dt)}  
% \end{align}
% \end{lemma}
% \begin{proof}
% In \cref{lem:exists}, we have seen that one of the desired encoders  $p(Z^*|X)$ is s.t. \cref{eq:lem_min_risk} holds, as a result all other desired encoders must achieve the same risk.
% \end{proof}

The following lemma essentially says that when $\risk{Y}{Z}$ is minimized, then the Bayes predictors for each domain all agree on the intersection of their support.

\ydnote{This lemma is quite hard to read due to the a.s.
For discrete that would simply give $\risk{Y}{Z} = \risk{Y}{X}$ implies
$\forall f_*^{d} \in \funcfamily_{d}^*, \ \forall z \in \supp{p(Z|d)}$ we have $f_*^{d}(z) = f_*(z) $
}
\begin{lemma}\label{lemm:agree}
$\risk{Y}{Z} = \risk{Y}{X}$ implies that for all $ f_*^{D} \in \funcfamily_{D}^*$ we have $f_*^{D}(Z') = f_*(Z') $ almost surely over $p(D)$ and over any $p(Z')$ s.t. $\supp{p(Z')} = \supp{p(Z|D)}$.
\end{lemma}
\begin{proof}
First let us show that $f_*(Z) \aseq f_*(X)$ when $\risk{Y}{Z} = \risk{Y}{X}$. Indeed:
\begin{align}
\risk{Y}{X} 
&\defeq \E{\dens{X, Y}}{\ell(Y, f_*(X))} \\
&= \E{\dens{X}}{\E{\conddens{Y}{X}}{\E{\conddens{Z}{X}}{\ell(Y, f_*(X))}}} \\
&= \E{\dens{X,Z}}{\E{\conddens{Y}{X}}{\ell(Y, f_*(X))}} 
\end{align}
\yrnote{This seems not super clear because $f^*$ is defined in on the $X$ space, did we define it for $Z$ space somewhere?}
As $\ell$ is a meaningful loss (\cref{asmp:losses}) we have that $\risk{Y}{X} = \risk{Y}{Z}$ if and only if the Bayes predictors $f_*(X) = f_*(Z)$ almost surely over $p(X,Z)$.
By the same computation for a specific domain we have $f_*^D(X) = f_*^D(Z)$ almost surely over $p(X,Z,D)$.
Using the invariance of the Bayes predictor from $X$ (\cref{asmp:bayes_inv}) we conclude that $f_*(Z) = f_*(X) = f_*^D(X) = f_*^D(Z)$ a.s. over $p(X,Z,D)$. 

So $f_*(Z) = f_*^D(Z)$ a.s. over $p(Z,D)$ for any Bayes predictor.
From which we conclude, as desired, that $f_*(Z') = f_*^D(Z')$ a.s. over $p(D)$ and over any $p(Z')$ s.t. $\supp{p(Z')} = \supp{p(Z|D)}$.

\end{proof}

\ydnote{Use manualthm instead to repeat the same number as in text (for some reason not working right now)}
\begin{theorem}[Characterizing optimal representations]
Under our assumptions, an encoder $p(Z^* \cond X) $ is optimal for domain generalization if and only if it minimizes the Bayes risk while matching the support of $\rv Z^*$ almost surely over $p(\Ds,\Dt)$, \ie, 
\begin{align}
p(Z^* \cond X) \in  & \arginf_{p(Z \cond X)} \quad \risk{Y}{Z} \label{eq:appx_min_risk}   \\
& \subject \quad \supp{p(Z \cond \Ds)} \aseq \supp{p(Z \cond \Dt)}  \label{eq:appx_support_match}  
\end{align}
\end{theorem}
\begin{proof}
Notice that the optimal DG Risk is lower bounded by $\risk{Y}{X}$. 
Indeed, 
\begin{align}
lhs &\defeq \inf_{\conddens{Z}{X}} \E{\dens{\Ds, \Dt}}{  \sup_{f \in \funcfamily_{\Ds}^* }  \domriskq{Z}{f}{\Dt}} \\
&\geq \inf_{\conddens{Z}{X}} \E{\dens{\Ds, \Dt}}{  \inf_{f \in \funcfamily_{\Ds}^* }  \domriskq{Z}{f}{\Dt}} \label{eq:geq_inf}\\
&= \inf_{\conddens{Z}{X}} \E{\dens{\Ds, \Dt}}{ \domrisk{Z}{\Dt}}  &   f_* \in \funcfamily_{\Ds}^* \\
&= \inf_{\conddens{Z}{X}} \risk{Y}{Z} \\
&\geq \risk{Y}{X} & \text{\cref{lem:DPI}} \label{eq:geq_RYX}
\end{align}
where the last inequality uses the DPI of Bayes risk.
We will now show that this lower bound is achieved by an encoder IFF it satisfies \cref{eq:appx_min_risk}  and \cref{eq:appx_support_match}. Such encoder always exist by \cref{lem:exists}.

\textbf{Sufficiency} ($\impliedby$):
Let $\conddens{Z}{X}$ be an encoder that satisfies \cref{eq:appx_min_risk}  and \cref{eq:appx_support_match}.
Then we have the following DG risk
\begin{align}
 lhs  &\defeq \E{p(\Ds,\Dt)}{\sup_{f \in \funcfamily_{\Ds}^*} \E{\conddens{Z,Y}{\Dt}}{\ell(Y,f(Z))}}  & \text{def.} \\
  &=
 \E{p(\Ds,\Dt)}{\sup_{f \in \funcfamily_{\Ds}^*} \E{\conddens{Z,Y}{\Dt}}{\ell(Y,f_*(Z))}} & \text{\cref{lemm:agree}} \label{eq:proof:agree} \\
  &=
 \E{p(\Dt)}{ \E{\conddens{Z,Y}{\Dt}}{\ell(Y,f_*(Z))}} & \text{constant w.r.t $\Ds$} \label{eq:proof:const} \\
  &=
 \E{p(D)}{ \E{\conddens{Z,Y}{D}}{\ell(Y,f_*(Z))}} & \text{\cref{asmp:domains}} \\
  &\eqdef
\risk{Y}{X}  
\end{align}
\Cref{eq:proof:agree} uses the a.s. equality of the supports (\cref{eq:appx_support_match}) and $\min \risk{Y}{Z} = \risk{Y}{X}$ (\cref{lem:min_risk} and \cref{eq:appx_min_risk}) to conclude that any Bayes optimal predictor on source a.s. predicts like the Bayes optimal predictor on all domains (\cref{lemm:agree}).


\textbf{Necessity} ($\implies$):
For the DG risk to be $\risk{Y}{X}$ we need both inequalities \cref{eq:geq_RYX} and \cref{eq:geq_inf} to be equalities.
To satisfy the latter, we need $\risk{Y}{Z} = \risk{Y}{X}$.
To satisfy the former inequality, we need
$ \sup_{f \in \funcfamily_{\Ds}^* }  \domriskq{Z}{f}{\Dt} =  \inf_{f \in \funcfamily_{\Ds}^* }  \domriskq{Z}{f}{\Dt}$ almost surely over $p(\Ds,\Dt)$.
We will prove by contrapositive that this implies support match (\cref{eq:appx_support_match}).
Suppose that the support match does not hold and denote as $S$ the event $Z \in \supp{\conddens{Z}{\Ds}}$ and $\bar{S}$ its complement, then with probability non-zero over $p(\Ds,\Dt)$ we have
\begin{align}
lhs &\defeq \sup_{f \in \funcfamily_{\Ds}^* }  \domriskq{Z}{f}{\Dt} \\
&= \sup_{f \in \funcfamily_{\Ds}^* }  p(S) \E{\conddens{Y,Z}{S,\Dt}}{l(Y,f(Z))} + p(\Bar{S}) \E{\conddens{Y,Z}{\Bar{S},\Dt}}{l(Y,f(Z))}  &\text{split supp} \\
&= \sup_{f \in \funcfamily_{\Ds}^* }  p(S) \E{\conddens{Y,Z}{S,\Dt}}{l(Y,f_*(Z))} + p(\Bar{S}) \E{\conddens{Y,Z}{\Bar{S},\Dt}}{l(Y,f(Z))} & \text{\cref{lemm:agree}}  \label{eq:proof:agree2} \\
&=  p(S) \E{\conddens{Y,Z}{S,\Dt}}{l(Y,f_*(Z))} + \sup_{f}  p(\Bar{S}) \E{\conddens{Y,Z}{\Bar{S},\Dt}}{l(Y,f(Z))} \label{eq:proof:sup}    \\
&=  p(S) \E{\conddens{Y,Z}{S,\Dt}}{l(Y,f_*(Z))} +  p(\Bar{S}) \E{\conddens{Y,Z}{\Bar{S},\Dt}}{l(Y,f_*(Z))} \nonumber \\
&\quad - 
p(\Bar{S}) \E{\conddens{Y,Z}{\Bar{S},\Dt}}{l(Y,f_*(Z))} +
p(\Bar{S}) \sup_{f}   \E{\conddens{Y,Z}{\Bar{S},\Dt}}{l(Y,f(Z))}  & \text{add }0 \\
&=  \inf_{f \in \funcfamily_{\Ds}^* }  \domriskq{Z}{f}{\Dt} +
p(\Bar{S}) \sup_{f}  \E{\conddens{Y,Z}{\Bar{S},\Dt}}{l(Y,f(Z)) - l(Y,f_*(Z))} \label{eq:proof:inf}  \\
&> \inf_{f \in \funcfamily_{\Ds}^* }  \domriskq{Z}{f}{\Dt} &\text{\cref{asmp:losses}} \label{eq:proof:non_zero}
\end{align}
\Cref{eq:proof:agree2} uses the Bayes predictor when the support matches due to \cref{lemm:agree}, which holds because $\risk{Y}{Z} = \risk{Y}{X}$ has to be satisfied due to \cref{eq:geq_inf}.
\Cref{eq:proof:sup} uses the fact that functions in $\funcfamily_{\Ds}^*$ are unconstrained outside of the support $\supp{p(Z | \Ds)}$.
\Cref{eq:proof:inf} uses the fact that the Bayes predictor $f_*$ is optimal on all domains due to \cref{asmp:bayes_inv}.
\Cref{eq:proof:non_zero} uses 
\begin{inlinelist}
\item that $\ell$ is a meaningfull loss (\cref{asmp:losses}) so $\E{\conddens{Y,Z}{\Bar{S},\Dt}}{l(Y,f(Z)) - l(Y,f_*(Z))}$ is strictly positive;
\item that $p(\Bar{S}) \geq 0$ because the support does not match by assumption.
\end{inlinelist}
We conclude that the inequality \cref{eq:geq_RYX} is not an equality when \cref{eq:appx_support_match} does not hold. 
By contrapositive we thus have that the support match must hold.
As we must also have $\risk{Y}{Z} = \risk{Y}{X}$ (\cref{eq:geq_inf}) we conclude using \cref{lem:min_risk} that \cref{eq:appx_min_risk} must also hold.
So both \cref{eq:appx_min_risk} and \cref{eq:appx_support_match} are necessary.
\end{proof}


As a corollary from the proof strategy we directly have that the optimal DG risk is simply $\risk{Y}{X}$. This is very interesting (and somewhat surprising) as it shows that using the optimal encoder one can actually perform just as well by training on the source than if you were to directly train on the target using the raw data. 

\begin{corollary}[Optimal DG Risk]
$\risk{Y}{X} = \inf \quad \E{p(\Ds,\Dt)}{\sup_{f \in \funcfamily_{\Ds}^*} \domriskq{Z}{f}{\Dt}}  $
\end{corollary}


\subsection{Constrained Functional Family}

We have previously studied the case of unconstrained predictive family.
Let us now consider the case of a constrained family of predictors $\mathcal{Q} \in \set{q : \mathcal{Z} \to \mathcal{A}}$.
We will make the following assumption which ensures that one can predict as well as possible.
\ydnote{Instead of adding other (possibly unrealistic) assumptions on Q I think we should just prove implication rather than IFF for constrained.}

\begin{assumption}[Non-empty preimage of Bayes image]\label{asmp:non_empty}
We consider the functional family $\mathcal{Q}$ that contains at least one predictor whose preimages of all Bayes images is non-empty. 
Formally $\exists q \in \mathcal{Q}, \forall a \in \mathcal{A}_*, \exists z \in \mathcal{Z}$ s.t. $q(y|z) = 1$.
\end{assumption}

Note that \cref{asmp:non_empty} generalizes previous assumptions made when when working with functional families for optimal representations.
Specifically, it recovers \citepos{dubois_learning_2020} Assumption of non-empty pre-image for the case of accuracy (or log loss with deterministic labels as they do).

We can now show that optimizing our objective also gives rise to an optimal encoder under the constrained predictors.
\begin{proposition}[Constrained predictors]
Let $\mathcal{Q}$ be a set of allowed predictors that satisfies \cref{asmp:non_empty}. Then optimizing our loss is still optimal, \ie, any encoder $p(Z|X)$ such that
\begin{align}\label{eq:constrained_Q}
p(Z|X) \in & \argmin_{p(Z \cond X)} \quad \riskQ{Y}{Z}   \\
& \subject \quad \supp{p(Z \cond \Ds)} \aseq \supp{p(Z \cond \Dt)}  
\end{align}
is also optimal and there always exist such encoder.
\end{proposition}
\begin{proof}
Construct the same encoder as in \cref{lem:exists}, which is possible because the preimage of $\mathcal{A}_*$ is non empty due to \cref{asmp:non_empty}.
As a result we have that such encoder exists and all encoders that satisfy our loss will (by \cref{lem:min_risk} and \cref{thm:main}) also be optimal.
\end{proof}

Note that contrary to the case of unconstraiend predictors our loss is only \textit{sufficient} for optimality but is not necessary. 
Intuitively, the reason this is the case is that there might can be very constrained predictors (say linear) s.t. even if the support of the representation does not match the worst case predictor will not be able to ``take advantage'' of a mismatch in the support.
\ydnote{Actually I have ideas as to how to do it but (1) takes time; (2) not that realistic. SO skipping}
We believe that this can be solved by adding new assumptions but we leave it for future work to do so.


\input{appendix/theory_augmentations}
