# Supplementary material for: Optimal Representations for Covariate Shift
Source: arXiv:2201.00057 source file (2022-03-14)
Supplement: Supplementary file 5 [file theory_old.tex]

\section{Theories and Proofs}
In this section, we include our theoretical results with detailed proofs.

\subsection{Main Theorem}
Here we first present the main theorem presented of our paper: 
\yrnote{will move to main body}


\begin{theorem}[Full Theorem]
Any encoder $\conddens{Z}{X}$ achieves the minimum of \cref{eq:full_gen_risk_obj} if and only if it achieves the minimum of the following problem:
\begin{align}
& \min_{\conddens{Z}{X}} \quad \riskQ{Y}{Z} \label{eq:full_iff_min_risk}   \\
& \subject \quad \supp{\dens{Z_{\ds}}}=\supp{\dens{Z_{\dt}}}, \forall{\ds, \dt \in \domspace}  \label{eq:full_iff_support_match}  
\end{align}
\end{theorem}

\begin{remark}
In fact, we will show that the minimum of \cref{eq:full_iff_min_risk} under the constraint \cref{eq:full_iff_support_match} can still achieve the (unconstrained) best possible risk, i.e., $\inf_{\conddens{Z'}{X}} \riskQ{Y}{Z'}$. Thus the optimality condition can also be rewritten as two constraints: 
\begin{gather}
    \riskQ{Y}{Z} = \inf_{\conddens{Z'}{X}} \riskQ{Y}{Z'} \\
    \supp{\dens{Z_{\ds}}}=\supp{\dens{Z_{\dt}}}, \forall{\ds, \dt \in \domspace}
\end{gather}
which forms the starting point our proof strategy. But we still keep the optimization form as in \cref{eq:full_iff_min_risk} because it leads to the practical optimization for achieving the optimal representations.
\end{remark}

In the following subsections, we prove this theorem in two cases with some additional assumptions: deterministic and stochastic labels $Y$, respectively.

\subsection{Deterministic Case}
We start with the deterministic label case with the following additional assumptions.
\begin{assumption}[Deterministic labels]
The label $Y$ is a deterministic function of the input $X$. More precisely, there exits a deterministic labeling function (which needs to align across domains by \cref{asmp:covariate_shift}) $t:\inputspace \to \labelspace$ s.t. $Y=t(X)$. Thus, $\conddens{Y}{X}(y \cond x)=\indicate{y=t(x)}$ and $\CH{Y}{X}=0$ due to discreteness of labels (\cref{asmp:discrete_label}).
\end{assumption}

\begin{assumption}[Same label set]\label{asmp:same_label_set}
\yrnote{change this to same label set instead of label space cover, for compatibility with the stochastic case.}
We assume that all the domains share the same label support, i.e., $\forall{d \in \domspace}, \supp{\dens{Y_d}}=\labelspace_s \subseteq \labelspace$. Equivalently, $\forall{d \in \domspace}, \forall{y \in \labelspace_s}, \dens{Y_d}(y) > 0$ and $\forall{y \not\in \labelspace_s}, \dens{Y_d}(y) = 0$. This assumption is made to ensure the existence of optimal representation in the deterministic case (\cref{lem:determn_exist}) and is generally true in practice and also in common benchmarks for domain shift, where the label support is typically the entire label space, i.e., $\labelspace_s=\labelspace$.
\end{assumption}

\begin{assumption}[Non-empty preimage of deterministic labels]\label{asmp:nonempty_preimage_label}
We consider the functional family $\funcfamily$ that contains at least one predictor whose preimages of all deterministic labels are non-empty. Formally, $\exists q \in \funcfamily, \forall y \in \labelspace, \exists z \in \repspace, q(y \cond z)=1$. This assumption is made also to ensure the existence of optimal representation in the deterministic case (\cref{lem:determn_exist}). It is usually true in most ML scenarios, for example, can be achieved by scaling the weights of the layer before softmax to very large (or equivalently, setting the temperature of softmax to very low) to obtain nearly determinisitic predictions for neural networks. 
This assumption is standard when working with functional families for optimal representations \tocite{}.
\end{assumption}



\begin{proposition}[Simplified Theorem with Deterministic Labels]\label{thm:determn_case}
(Under above assumptions) Any encoder $\conddens{Z}{X}$ that achieves the minimum of the following objective ($=0$):
\begin{align} \label{eq:determn_gen_risk_obj}
    \inf_{\conddens{Z}{X}} \quad 
    & \E{\dens{\Ds, \Dt}}{  \sup_{q \in \funcfamily_{\Ds}^* } \riskq{Y_{\Dt}}{Z_{\Dt}}{q}}
\end{align}
if and only if:
\begin{gather} 
\riskQ{Y}{Z} = \inf_{\conddens{Z'}{X}} \riskQ{Y}{Z'} = 0  \label{eq:determn_iff_zero_risk}  \\
\supp{\dens{Z_{\ds}}}=\supp{\dens{Z_{\dt}}}, \forall{\ds, \dt \in \domspace} \label{eq:determn_iff_support_match}  
\end{gather}
\end{proposition}

The following lemma is a simple adaptation of the proof from \citet{dubois2020dib} Proposition 6 . 
% \ydnote{I'm adding these sentences. It's actually not only because it's DIB: I feel very strongly about being always very clear what is novel in that work and what comes from other papers :). Also we should always relate if possible all our new results to previous results in the literature (like ``this is a generalization of X when Y'').
% As a reviewer this is something I'd get very annoyed about if not done (even if it's a result I know about but not my paper).
% }

\begin{lemma}[Existence]\label{lem:determn_exist}
There exists encoder $\conddens{Z}{X}$ s.t. \cref{eq:determn_iff_zero_risk} and \cref{eq:determn_iff_support_match} are satisfied.
\end{lemma}
\begin{proof}
This can be proved by construction by using the same strategy as in the proof of \citet{dubois2020dib} Proposition 6, but ensuring that such encoder exists when $\mathcal{Z}$ is not finite.
Intuitively, they split $\repspace$ according to $\labelspace$ and let $\conddens{Z}{X}$ map each $X$ uniformly over split corresponding to its deterministic $Y$. The same proof holds when uniform distributions cannot be defined as we now show.
    
Formally, with \cref{asmp:nonempty_preimage_label}, we have a predictor $q \in \funcfamily$ such that $\forall y \in \labelspace$, $\exists z \in \repspace$, it \emph{deterministically} predicts the label $y$ from $z$, i.e., $q(y \cond z)=1$. Denote the preimage of the deterministic prediction $y$ by the predictor $q$ as $q^{\leftarrow}(y)=\{z : q(y \cond z)=1, z \in \repspace \}$, the assumption implies $\forall y \in \labelspace, |q^{\leftarrow}(y)|>0$. 
% We can simply construct an encoder to map the input $x \in \inputspace$ to a uniform distribution over the preimage of the deterministic label $t(x)$:
% \begin{equation}
%     \conddens{Z}{X}(z|x)=
%     \begin{cases}
%         \frac{1}{|q^{\leftarrow}(t(x))|} & z \in q^{\leftarrow}(t(x)) \\
%         0 & \mathrm{otherwise}
%     \end{cases}
% \end{equation}
We can simply construct an encoder to map the input $x \in \inputspace$ to any valid distribution whose support is the preimage of its deterministic label $q^{\leftarrow}(t(x))$, i.e., $\supp{\conddens{Z}{x}}=q^{\leftarrow}(t(x))$.
% \ydnote{
% This doesn't hold in countable infinite $\mathcal{Z}$ case: there exists no unifrom distribution over any countably infinite sample space.
% This also doesn't always work if $\rv Z$ is continuous. 

% I would just say ``We can simply construct an encoder to map the input $x \in \inputspace$ to a any valid distribution whose support is the preimage of the deterministic label $q^{\leftarrow}(t(x))$''.

% For DIB I only worked with finite sample space for other reasons. But we definitely shouldn't do that.
% }
It is easy to show that for such $Z$, $\riskQ{Y}{Z}=\riskq{Y}{Z}{q}=0$ due to the fact that $\forall{x \in \inputspace}$, $\forall{z \in \supp{\conddens{Z}{x}}}$, we have $q(t(x) \cond z)=1$, which leads to \cref{eq:determn_iff_zero_risk}. Furthermore, $\forall{d \in \domspace}$, the support of the constructed $Z$ is $\bigcup_{y \in \supp{\dens{Y_d}}} q^{\leftarrow}(y)=\bigcup_{y \in \labelspace_s} q^{\leftarrow}(y)$ due to \cref{asmp:same_label_set} and is the same for all domains, thus we have shown that \cref{eq:determn_iff_support_match} is also satisfied. 
\end{proof}

\begin{lemma}\label{lem:determn_zero_risk_meaning}
\cmnote{The proof of this is very hard to follow and needs to be cleaned up. I also want us to get rid of the best case analysis. I think it's very distracting and we can do it as a remark.}
The following two conditions are equivalent:
\begin{enumerate}
    \item $\riskQ{Y}{Z} = 0$ \label{item:cond_overall}.
    \item Conditions include \ydnote{what do you mean by ``conditions include''}    \label{item:cond_split}
    \begin{enumerate}
        \item $\forall d \in \mathcal{D}, \riskQ{Y_d}{Z_d}=0$ \label{item:cond_split_sufficiency}.
        \item The functional family contains the conditional $\conddens{Y}{Z}$, i.e., $\exists \qstar \in \funcfamily, \qstar\condalign\conddens{Y}{Z}$ \label{item:cond_split_include_cond}.
        % \ydnote{this is equal not align, ie, $\qstar = \conddens{Y}{Z}$, because both are defined on same domain $\mathcal{Z}$}
        \item The conditionals $\conddens{Y_d}{Z_d}$ align across domains, i.e., $\conddens{Y}{Z} \condalign \conddens{Y_d}{Z_d}$ for all $d \in \domspace$. \label{item:cond_split_cond_inv}
    \end{enumerate}
\end{enumerate}
Both these two conditions lead to the optimal \emph{best-case} generalization risk ($=0$):
\begin{equation} \label{eq:determn_best_case}
    \E{\dens{\Ds, \Dt}}{  \inf_{q \in \funcfamily_{\Ds}^* } \riskq{Y_{\Dt}}{Z_{\Dt}}{q}}=0
\end{equation}
% $\riskQ{Y}{Z} = 0$ $\overset{(a)}{\iff}$ $\forall d \in \mathcal{D}, \riskQ{Y_d}{Z_d}=0$ and $\conddens{Y}{Z}$ is invariant across domains $\exists \qstar \in \funcfamily$ such that $\qstar\condalign\conddens{Y}{Z}$ and is optimal for all domains
% % , i.e., $\riskq{Y_d}{Z_d}{\qstar}=\riskQ{Y_d}{Z_d}=0$ 
% $\overset{(b)}{\iff}$ $\E{\dens{\Ds, \Dt}}{  \inf_{q \in \funcfamily_{\Ds}^* } \riskq{Y_{\Dt}}{Z_{\Dt}}{q}}=0$.
\end{lemma}

% \yrnote{generalize to infinite or even continuous $D$?}
% \ydnote{I wouldn't. It's going to be overly complicated for the reader, essentially you won't be able to say $\forall d$, \eg, in the support condition. But something like ``the probability of having a z outside of the intersection of the supports is 0''.
% I would probably work with finite $\mathcal{D}$ and then say ``btw our optimal Z provides guarantees for any domains that ...''
% }

\begin{proof}
We first show the sufficiency and necessity between Cond. \ref{item:cond_overall} and Cond. \ref{item:cond_split}.
\cmnote{Sufficiency: Let $d_s$, $d_t$ be any pair of domains. By Lemma 2 and (17), we have that $q_{d_s}$ in $Q^*_{d_s}$ and $q_{d_t}$ in $Q^*_{d_t}$ agree (a.s.) with $p_{Y | Z}$ on the intersection of their support. Since their supports match exactly, we have that $q_{d_s}$ and $q_{d_t}$ agree a.s. and $R_{q_s}[Y_{d_t} | Z_{d_t}] = 0$. This means that (16) is minimized.}
Cond. \ref{item:cond_overall} $\implies$ Cond. \ref{item:cond_split}: Denote the optimal predictor as $\qstar \in \funcfamily$, we have $\riskQ{Y}{Z}=\riskq{Y}{Z}{\qstar}=0$. Since 
\begin{equation}
    \riskq{Y}{Z}{\qstar} \geq \CH{Y}{Z} \geq 0
\end{equation}
with equalities hold only if $\CH{Y}{Z}=0$ and $\qstar \condalign \conddens{Y}{Z}$
\ydnote{actually it only needs to align almost surely }
(Cond. \ref{item:cond_split_include_cond}) due to the strict properness of log loss \citep{gneiting2007strictly}. Furthermore, if we split the risk over domains,
\begin{equation}
    \riskq{Y}{Z}{\qstar}=\E{\dens{D}}{\riskq{Y_{D}}{Z_{D}}{\qstar}}
    \geq \E{\dens{D}}{\riskQ{Y_{D}}{Z_{D}}}
    \geq \E{\dens{D}}{\CH{Y_{D}}{Z_{D}}} \geq 0
\end{equation}
with equalities only hold if $\riskq{Y_d}{Z_d}{\qstar}=\riskQ{Y_d}{Z_d}=\CH{Y_d}{Z_d}=0$, $\forall{d \in \domspace}$ (with \cref{asmp:finite_domain} and \cref{asmp:cover_domains}), which leads to Cond. \ref{item:cond_split_sufficiency}. This also implies that $\qstar \condalign \conddens{Y_d}{Z_d}$ and by transitivity we have $\conddens{Y}{Z} \condalign \conddens{Y_d}{Z_d}, \forall{d \in \domspace}$, which means $\conddens{Y_d}{Z_d}$ agree across domains (Cond. \ref{item:cond_split_cond_inv}) and $\qstar$ achieves optimality for all domains.
% \ydnote{no need transitivity here because $\qstar = \conddens{Y}{Z}$ not align.}
\ydnote{Honestly quite hard to follow the writing style...}
\yrnote{definitely need to clean up more..}

\cmnote{Necessity. This is very hard to follow and show be cleaned up. The order of arguments is a bit convoluted. You should think of a proof as a directed acyclic graph where the root are the assumptions and the leaves are the things you're trying to prove. The parent-child relationship is an implication in the proof. Taking this view, the parent should always come before the child and you should try to find the DAG with a small number of nodes. My feeling is that this was not done for the argument below (maybe wrong)}
\cmnote{Necessity for continuous $Z$. I think our statement is incorrect for continuous Z. What we need is that symmetric difference of the supports is a set of measure 0 w.r.t the base measure, not what we have here.}
Cond. \ref{item:cond_overall} $\impliedby$ Cond. \ref{item:cond_split}: Since we have $\conddens{Y}{Z} \condalign \qstar \in \funcfamily$ and $\forall{d \in \domspace}, \conddens{Y}{Z} \condalign \conddens{Y_d}{Z_d}$, we have $\qstar \condalign \conddens{Y_d}{Z_d}$ by transitivity.
% \ydnote{again no need transitivity}
It implies that $\qstar$ is optimal for domains, i.e., $\riskq{Y_d}{Z_d}{\qstar}=\riskQ{Y_d}{Z_d}=0, \forall{d \in \domspace}$ due to the strict properness of log loss. 
% \yrnote{we need to have a lemma for strict properness?}
% \ydnote{no but you need to cite \url{https://www.tandfonline.com/doi/abs/10.1198/016214506000001437} the first time}
Thus we have 
\begin{equation}
    \riskq{Y}{Z}{\qstar}=\E{\dens{D}}{\riskq{Y_{D}}{Z_{D}}{\qstar}}=0
\end{equation}
Since $\riskq{Y}{Z}{\qstar} \geq \riskQ{Y}{Z}$, we have $\riskQ{Y}{Z}=0$ due to the non-negativity of log loss with discrete $Y$.
% \ydnote{and positivity of log loss risk due to discreteness of $Y$}

Finally we show that Cond. \ref{item:cond_split} leads to \cref{eq:determn_best_case} satisfied. Similar to the previous analysis, from Cond. \ref{item:cond_split}, we have that $\conddens{Y}{Z} \condalign \qstar \in \funcfamily$ is optimal for all domains. Then $\forall \ds, \dt \in \domspace$, we have $\qstar \in \funcfamily^*_{\ds}$ and $\riskq{Y_{\dt}}{Z_{\dt}}{\qstar} = \riskQ{Y_{\dt}}{Z_{\dt}} = 0$. Thus we have $\inf_{q \in \funcfamily_{\ds}^* } \riskq{Y_{\dt}}{Z_{\dt}}{q} = \riskq{Y_{\dt}}{Z_{\dt}}{\qstar}=0$. Taking expectation over the randomly selected $\Ds, \Dt$, we have $\E{\dens{\Ds, \Dt}}{  \inf_{q \in \funcfamily_{\Ds}^* } \riskq{Y_{\Dt}}{Z_{\Dt}}{q}}=0$.


% Cond. \ref{item:cond_split} $\impliedby$ Cond. \ref{item:cond_best_case}: From Cond. \ref{item:cond_best_case}, with \cref{asmp:finite_domain} and \cref{asmp:cover_domains}, we have $\inf_{q \in \funcfamily_{\ds}^* } \riskq{Y_{\dt}}{Z_{\dt}}{q}=0$ for $\forall{\ds, \dt \in \domspace}$. Then, 
% \begin{equation}
%     \inf_{q \in \funcfamily_{\ds}^* } \riskq{Y_{\dt}}{Z_{\dt}}{q}
%     \geq \inf_{q \in \funcfamily} \riskq{Y_{\dt}}{Z_{\dt}}{q} 
%     = \riskQ{Y_{\dt}}{Z_{\dt}}
% \end{equation}
% which leads to the fact that Cond. \ref{item:cond_split_sufficiency} due to the non-negativity of log loss. Since $\riskQ{Y_{\dt}}{Z_{\dt}}$ achieves the infimum and with the strict properness of log loss, we know that $\forall \dt \in \domspace$, $\exists \qstar_{\dt} \in \funcfamily$ such that $\qstar_{\dt} \condalign \conddens{Y_{\dt}}{Z_{\dt}}$. 
% Finally, we show $\forall \dt \in \domspace, \conddens{Y}{Z} \condalign \conddens{Y_{\dt}}{Z_{\dt}}$ by contradiction. 

\end{proof}

% \begin{lemma}
% Under covariat shift, best = worst $\iff$ support match.
% \end{lemma}


% \ydnote{I would still have a an additional lemma here for worst case. 
% i.e. lemma 3: under \cref{eq:determn_iff_zero_risk} we have $inf=sup$ if and only if 
% \cref{eq:determn_iff_support_match}.

% Then the proof of proposition 1 is only: 
% - the  \cref{eq:determn_gen_risk_obj} $\geq$ 0 by definition
% - from lemma 1,2,3 we know that there exists a $\rv Z$ such that \cref{eq:determn_gen_risk_obj} $= 0$ 
% - we conclude that all optima have $sup=inf=0$ which by lemma 2 and 3 means that \cref{eq:determn_iff_support_match} and \cref{eq:determn_iff_zero_risk} hold.
% Honestly it's a little hard to follow the proof for now, and I think that more lemmas would help (+ give better intuition).
% }
\begin{proof}[Proof of \cref{thm:determn_case}]
We prove the sufficiency and necessity of the optimality conditions separately.


Sufficiency ($\impliedby$): From \cref{lem:determn_zero_risk_meaning}, we have that \cref{eq:determn_iff_zero_risk} leads to the optimal best-case generalization risk, i.e., \cref{eq:determn_best_case}. Then we show that \cref{eq:determn_iff_support_match} leads to the fact that the worst case is the same as the best case, i.e.,
\begin{equation}\label{eq:determn_worst_eq_best}
    \E{\dens{\Ds, \Dt}}{  \sup_{q \in \funcfamily_{\Ds}^* } \riskq{Y_{\Dt}}{Z_{\Dt}}{q}} = \E{\dens{\Ds, \Dt}}{  \inf_{q \in \funcfamily_{\Ds}^* } \riskq{Y_{\Dt}}{Z_{\Dt}}{q}}
\end{equation}
We show this by contrapositive: assume that the above equation is not satisfied, then $\exists \ds, \dt \in \domspace$ such that $\sup_{q \in \funcfamily_{\ds}^* } \riskq{Y_{\dt}}{Z_{\dt}}{q} > \inf_{q \in \funcfamily_{\ds}^* } \riskq{Y_{\dt}}{Z_{\dt}}{q}$. This implies that $\exists \qstar_1, \qstar_2 \in \funcfamily^*_{\ds}$ such that $\riskq{Y_{\dt}}{Z_{\dt}}{\qstar_1} \neq \riskq{Y_{\dt}}{Z_{\dt}}{\qstar_2}$. From \cref{lem:determn_zero_risk_meaning}, we know that $\qstar_1 \condalign \conddens{Y_{\ds}}{Z_{\ds}}$ and $\qstar_2 \condalign \conddens{Y_{\ds}}{Z_{\ds}}$ due to the strict properness of log loss, this leads to the fact that $\qstar_1(\vardot \cond z) = \qstar_2(\vardot \cond z), \forall{z \in \supp{\dens{Z_{\ds}}}}$. 
\ydnote{Why need strict properness here ? that's just lemma 2 right ?}
Then the fact that $\riskq{Y_{\dt}}{Z_{\dt}}{\qstar_1} \neq \riskq{Y_{\dt}}{Z_{\dt}}{\qstar_2}$ implies that $\exists z \in \supp{\dens{Z_{\dt}}} \not\in \supp{\dens{Z_{\ds}}}$ such that $\qstar_1(\vardot \cond z) \neq \qstar_2(\vardot \cond z)$, but this means $\supp{\dens{Z_{\dt}}} \setminus \supp{\dens{Z_{\ds}}} \neq \emptyset$, which contradicts \cref{eq:determn_iff_support_match}.

Necessity ($\implies$): We first show by contradiction that if \cref{eq:determn_gen_risk_obj} achieves the minimum ($=0$), then \cref{eq:determn_iff_support_match} must be satisfied. Assume that $\exists \ds, \dt \in \domspace$, $\supp{\dens{Z_{\ds}}} \neq \supp{\dens{Z_{\dt}}}$, without loss of generality, we assume that $\supp{\dens{Z_{\dt}}} \setminus \supp{\dens{Z_{\ds}}} \neq \emptyset$, then for $\forall \qstar_{\ds} \in \funcfamily^*_{\ds}$, $\forall{z \in \supp{\dens{Z_{\dt}}} \setminus \supp{\dens{Z_{\ds}}}}$, $\qstar_{\ds}(\vardot \cond z)$ can be arbitrary. Thus $\sup_{q \in \funcfamily_{\ds}^* } \riskq{Y_{\dt}}{Z_{\dt}}{q}$ is not predictable and must be larger than the minimum ($=0$)
\ydnote{this is not very formal ... need to be improved. I would probably do it by construction: show how to construct such q.
}
\yrnote{we need put some assumptions on functional family for this to be rigorous}.
\ydnote{Yes need to add. Maybe: there always exist a predictor that differs in only one $z$, \ie, $\forall z' \in \mathcal{Z}, \forall q, \exists q'$ such that $q(\cdot|z') \neq q'(\cdot|z')$ but $q(\cdot|z)=q'(\cdot|z)$ for all $z \neq z'$.
Then for the example chose $z'$ to be in the $d_t$ but not $d_s$ and conclude that $q'$ cannot also reach $0$.
}
\ydnote{I have to think more carefully about  continuous $\rv Z$ here. I think it works but will double check. THe issue is that what we really want is an almost sure statement which is less stringent than ``on the support'' (because the support has to be closed). But I think that when densities exist both of these statements are the same... I'll come back on that.
}
Then \cref{eq:determn_gen_risk_obj} must also be larger than $0$ (with \cref{asmp:finite_domain} and \cref{asmp:cover_domains}), which leads to a contradiction, thus we have shown that \cref{eq:determn_iff_support_match} must be satisfied.

Furthermore, \cref{eq:determn_gen_risk_obj} achieves the minimum ($=0$) implies that $\forall{\ds, \dt \in \domspace}$, we have $\sup_{q \in \funcfamily_{\ds}^* } \riskq{Y_{\dt}}{Z_{\dt}}{q}=0$ (with \cref{asmp:finite_domain} and \cref{asmp:cover_domains}). Based on this fact, we prove the necessity of \cref{eq:determn_iff_zero_risk} by showing the Cond. \ref{item:cond_split}, which directly follows \cref{lem:determn_zero_risk_meaning}.
\ydnote{What you are trying to achieve is not very clear. 
From what I uderstand you are trying to prove cond 2 which is equivalent \cref{eq:determn_iff_zero_risk} by lemma 2. Right now it's not clear.

Also I would change lemma 2 to show that inf is necessary (i.e. $inf=0$ is equivalent to the other 2 conditions).
Can you not just say: if $sup=0$ then $inf=0$ so by lemma 2 we need cond 1 which is \cref{eq:determn_iff_zero_risk}.
}
\begin{enumerate}
    \item By setting $\ds=\dt=\forall d \in \domspace$, we have $\riskQ{Y_d}{Z_d}=\sup_{q \in \funcfamily_{d}^* } \riskq{Y_{d}}{Z_{d}}{q}=0$, which leads to Cond. \ref{item:cond_split_sufficiency}. 
    \item For a fixed $\ds \in \domspace$, $\forall \qstar_{\ds} \in \funcfamily_{\ds}^*$, we have that $\forall{\dt \in \domspace}, \riskq{Y_{\dt}}{Z_{\dt}}{\qstar_{\ds}}=0$ and achieves the minimum. This implies $\forall{\dt \in \domspace}, \qstar_{\ds} \condalign \conddens{Y_{\dt}}{Z_{\dt}}$ due to the strict properness of log loss. By transitivity, we have that $\conddens{Y_d}{Z_d}$ align across domains, which leads to Cond. \ref{item:cond_split_cond_inv}.
    \ydnote{again not by transitivity}
    \item From \cref{eq:determn_iff_support_match}, we know that $\supp{\dens{Z}}$ is equal to $\supp{\dens{Z_{\ds}}}$ and thus $\conddens{Y}{Z}$ equals $\conddens{Y_{\ds}}{Z_{\ds}}$. This means that $\qstar_{\ds}\condalign\conddens{Y}{Z}$, which leads to Cond. \ref{item:cond_split_include_cond}.
\end{enumerate}
\end{proof}

\begin{remark}
Intuitively, perfect domain generalization (with $0$ generalization risk) requires the following three criterions which can be all satisfied in the deterministic case:
\ydnote{don't like ``sufficiency''. Maybe ``in domain decodability'' and ``cross domain decodablility'' ? not sure ...}
\begin{itemize}
    \item sufficiency: $\riskQ{Y_d}{Z_d}=0~ \forall d \in \mathcal{D}$.
    \item conditional alignment: $\forall{d \in \domspace}, \conddens{Y_d}{Z_d} \condalign \conddens{Y}{Z}$.
     \item decodability: $\exists q \in \funcfamily, q \condalign \conddens{Y}{Z}$.
    \item support match: $\supp{\dens{Z_{\ds}}}=\supp{\dens{Z_{\dt}}}, \forall{\ds, \dt \in \domspace}$.
\end{itemize}
\end{remark}

Note: intuitively, support match forces the representation to throw away domain variant features (spurious correlations).

\subsection{Stochastic Case}
For convenience, we introduce a pseudo label $Y' \in \distspace(\labelspace)$ and reinterpret the stochastic label setting: there exits a \emph{deterministic} labeling function (which needs to align across domains due to \cref{asmp:covariate_shift}) $t':\inputspace \to \mathcal{Y'}\defeq\distspace(\labelspace)$ s.t. $Y'=t'(X)$. Here $t'$ can be treated as a conditional distribution and $t' \condalign \conddens{Y}{X}$. The key intuition here is that the underlying task is to predict $Y'$ instead of $Y$ itself (in the optimal case).
% \todo{maybe needed regular conditional assumptions}
\begin{itemize}
    \item The prediction from $Z$ to $Y$ can be decomposed into 
    \begin{equation}
        Z \underbrace{\overset{q'}{\rightarrow} Y' \overset{\mathbb{I}}{\rightarrow}}_{q} Y
    \end{equation}
    Here $q':\repspace \to \mathcal{Y'}$ is the (deterministic) predictor from $Z$ to $Y'$. And $\mathbb{I}: \mathcal{Y'} \to \distspace(\labelspace)$ is the identity function (copy-paste), note that $\mathcal{Y'}\defeq\distspace(\labelspace)$.
    \item There exists a bijective mapping between $q$ and $q'$ with $q'(y' \cond z)=1$ where $y'=q(\vardot \cond z)$. More specifically, $\forall{z \in \repspace}$, $q(\vardot \cond z)=y' \iff q'(y' \cond z)=1$. And the functional family of $q'$ denoted as $\mathcal{Q'}$ is induced by $Q$, i.e., $\mathcal{Q'}=\{q': q'(y' \cond z)=1~\mathrm{where}~y'=q(\vardot \cond z)~\mathrm{for}~q \in \funcfamily\}$
\end{itemize}
\todo{change the meaning of Y'}
\ydnote{Yes change so that the second part is not copy past but lookup table. And first part is only a classification from 1 to $|\mathcal{Y}'|$
}

% \ydnote{say that all the previous assumptions are direct generalization of the previosu assumptions where you replace $\rv Y$ by $\rv Y'$}
Based on this observation, we can generalize the assumptions and theoretical results in the deterministic case, where we replace $Y$ with the pseudo deterministic label $Y'$:

\begin{assumption}[Countable conditionals]\label{asmp:count_conditional}
\yrnote{make this assumption more sensible}
We assume that the space of the conditionals (i.e., pseudo label space) $\labelspace'$ is countable (and finite???). This assumption is made to ensure that the pseudo label $Y'$ can be treated as discrete (and finite???) labels and thus we can use the same proof strategy as before.
\end{assumption}

\begin{assumption}[Same conditional set]\label{asmp:same_conditional_set}
We assume that all the domains share the same conditional set, i.e., $\{\conddens{Y}{x} | x \in \supp{\dens{X_d}} \}$ is the same for $\forall d \in \domspace$. Equivalently, the support of pseudo labels is the same across all domains, i.e., $\forall d \in \domspace, \supp{\dens{Y_d'}}=\labelspace'_s$. 
\end{assumption}

\begin{assumption}[Non-empty preimage of stochastic conditionals]\label{asmp:nonempty_preimage_consitional}
We consider the functional family $\funcfamily$ that contains at least one predictor whose preimages of all stochastic conditionals in the support (equivalently, deterministic pseudo labels) is non-empty. Formally, $\exists q \in \funcfamily, \forall y' \in \supp{\dens{Y'}}, \exists z \in \repspace, q(\vardot \cond z)=y'$. Note this implies that $\exists q' \in \funcfamily', \forall y' \in \supp{\dens{Y'}}, \exists z \in \repspace, q'(y' \cond z)=1$.
\end{assumption}

% \ydnote{need another assumption: to use the same proof strategy you need $\mathcal{Y}'$ to be countable right ? because $\rv Y'$ needs to be discrete.}
% \begin{gather} 
% \min \quad \riskq{Y}{Z}{q \in Q^*_{\Ds}} \\
% s.t.\quad \riskQ{Y_{\Ds}}{Z_{\Ds}} = \CH{Y_{\Ds}}{Z_{\Ds}}  \\
% s.t.\quad \supp{\dens{Z_{\Dt}}} \subseteq \supp{\dens{Z_{\Ds}}}, \forall{\Dt \in \domspace}
% \end{gather}

\begin{proposition}[Stochastic Case]\label{thm:stoc_case}
Any encoder $\conddens{Z}{X}$ that achieves the minimum of the following objective (=$0$):
\begin{align} \label{eq:stoc_gen_risk_obj}
    \inf_{\conddens{Z}{X}} \quad 
    & \E{\dens{\Ds, \Dt}}{  \sup_{q \in \funcfamily_{\Ds}^* } \riskq{Y_{\Dt}}{Z_{\Dt}}{q}-  \inf_{\conddens{Z'}{X}}\riskQ{Y_{\Dt}}{Z'_{\Dt}} } 
\end{align}
if and only if:\yrnote{maybe explain why $\inf_{\conddens{Z}{X}}\riskQ{Y}{Z'} = \CH{Y}{X}$}
\begin{gather}
\riskQ{Y}{Z} = \inf_{\conddens{Z}{X}}\riskQ{Y}{Z'} = \CH{Y}{X} \label{eq:stoc_iff_min_risk}   \\
\supp{\dens{Z_{\ds}}}=\supp{\dens{Z_{\dt}}}, \forall{\ds, \dt \in \domspace}  \label{eq:stoc_iff_support_match}  
\end{gather}
\end{proposition}

\begin{lemma}\label{lem:stoc_bijection_min}
For the bijection pair $q$ and $q'$, i.e., which satisfies that $\forall z \in \repspace, q(\vardot \cond z)=y' \iff q'(y' \cond z)=1$, we have that $\riskq{Y}{Z}{q}=\CH{Y}{X} \iff \riskq{Y'}{Z}{q'}=0$.
\end{lemma}
\begin{proof}
We prove this by explicitly writing out the form of $\riskq{Y}{Z}{q}$ and $\riskq{Y'}{Z}{q'}$.

First, for $\riskq{Y}{Z}{q}$, we have
\begin{equation}
    \begin{aligned}
        \riskq{Y}{Z}{q}
        &= \E{\dens{X}\conddens{Z}{X}\conddens{Y}{X}}{-\log q(Y \cond Z)}\\
        &\geq \E{\dens{X}\conddens{Z}{X}\conddens{Y}{X}}{-\log \conddens{Y}{X}(Y \cond X)}\\
        &= \E{\dens{X}\conddens{Y}{X}}{-\log \conddens{Y}{X}(Y \cond X)}\\
        &= \CH{Y}{X}
    \end{aligned}
\end{equation}
Due to the strict properness of log loss, $\riskq{Y}{Z}{q}=\CH{Y}{X}$ if and only if $\forall x \in \supp{\dens{X}}$, $\forall z \in \supp{\conddens{Z}{x}}$, $q(\vardot \cond z)=\conddens{Y}{x}=y'$. 

Similarly, for $\riskq{Y'}{Z}{q'}$, note that $Y'=t'(X)$, we have 
\begin{equation}
    \begin{aligned}
        \riskq{Y'}{Z}{q'} = \E{\dens{X}\conddens{Z}{X}}{-\log q'(Y' \cond Z)} \geq 0
    \end{aligned}
\end{equation}
Due to the strict properness of log loss, $\riskq{Y'}{Z}{q'}=0$ if and only if $\forall x \in \supp{\dens{X}}$, $\forall z \in \supp{\conddens{Z}{x}}$, $q'(y' \cond z)=1$.

Finally, we note that due to bijectivity, $q(\vardot \cond z)=y' \iff q'(y' \cond z)=1$, the above two conditions are equivalent and the proof is complete. 
\end{proof}


\begin{lemma}\label{lem:stoc_min_risk_meaning}
$\riskQ{Y}{Z}=\CH{Y}{X} \iff \riskq{Y'}{Z}{Q'}=0$. Furthermore, there's a bijective mapping between $Q^*$ and $Q'^*$.
\end{lemma}
\begin{proof}
This lemma is a direct result of \cref{lem:stoc_bijection_min}. 
If $\riskQ{Y}{Z}=\CH{Y}{X}$, then for $ q \in \funcfamily^*$, $\riskq{Y}{Z}{q}=\CH{Y}{X}$. By \cref{lem:stoc_bijection_min}, we know that its bijective map $q' \in \funcfamily'$ satisfies that $\riskq{Y'}{Z}{q'}=0$, thus $\riskq{Y'}{Z}{Q'}=0$ and $q' \in \funcfamily'^*$ with the fact that $\riskq{Y'}{Z}{Q'} \geq 0$. 
Similarly, we can show the other way around: If $\riskq{Y'}{Z}{Q'}=0$, then for $ q' \in \funcfamily'^*$, $\riskq{Y'}{Z}{q'}=0$. By \cref{lem:stoc_bijection_min}, we know that its bijective map $q \in \funcfamily$ satisfies that $\riskq{Y}{Z}{q}=\CH{Y}{X}$, thus $\riskQ{Y}{Z}=\CH{Y}{X}$ and $q \in \funcfamily^*$ with the fact that $\riskQ{Y}{Z} \geq \CH{Y}{X}$. Now we have completed the proof.
\end{proof}

\begin{lemma}[Existence]\label{lem:stoc_exist}
There exits encoder $\conddens{Z}{X}$ s.t. \cref{eq:stoc_iff_min_risk} and \cref{eq:stoc_iff_support_match} are satisfied.
\end{lemma}
\begin{proof}
From \cref{lem:stoc_min_risk_meaning}, we just need to show that There exits encoder $\conddens{Z}{X}$ s.t. $\riskq{Y'}{Z}{Q'}=0$ and \cref{eq:stoc_iff_support_match} is satisfied. Note that these two conditions are almost the same as those in \cref{lem:determn_exist}, except that $Y'$ and $Q'$ are used instead of $Y$ and $Q$. Then with \cref{asmp:same_conditional_set} and \cref{asmp:nonempty_preimage_consitional}, we can use a similar construction strategy that splits $\repspace$ according to the pseudo label $Y'$ to prove the existence.
\end{proof}

\begin{proof}[Proof of \cref{thm:stoc_case}]
We first show that in the \emph{optimal} case, any encoder that achieves the minimum of \cref{eq:stoc_gen_risk_obj} ($=0$) if and only if it achieves the minimum ($=0$) of the following objective:
\begin{align} \label{eq:stoc_gen_risk_obj_pseudo}
    \inf_{\conddens{Z}{X}} \quad 
    & \E{\dens{\Ds, \Dt}}{  \sup_{q' \in \funcfamily_{\Ds}^{'*} } \riskq{{Y'}_{\Dt}}{Z_{\Dt}}{q'}}
\end{align}
This is because that for such encoder, we must have $\forall q \in \funcfamily^*_{\Ds}$, $\riskq{Y_{\Dt}}{Z_{\Dt}}{q}=\inf_{\conddens{Z'}{X}}\riskQ{Y_{\Dt}}{Z'_{\Dt}}=\CH{Y_{\Dt}}{X_{\Dt}}$. By \cref{lem:stoc_min_risk_meaning}, $\forall q' \in \funcfamily'^*_{\Ds}$, we can find its bijective pair $q \in \funcfamily^*_{\Ds}$, and by \cref{lem:stoc_bijection_min}, we have $\riskq{Y'_{\Dt}}{Z_{\Dt}}{q'}=0$. Similarly, we can show the other way around and prove the equivalence. 

Then again by \cref{lem:stoc_min_risk_meaning}, we can replace \cref{eq:stoc_iff_min_risk} with $\riskq{Y'}{Z}{Q'}=0$. Now we reduce the stochastic case to the deterministic case (\cref{thm:determn_case}), with $Y$ and $Q$ replaced with $Y'$ and $Q'$ respectively, and the proof follows \cref{thm:determn_case}.
\end{proof}

\todo{Add a colory for domain gen}
